# Supplementary material for: Range, not Independence, Drives Modularity in Biologically Inspired Representations
Source: arXiv:2410.06232 source file (2025-04-11)
Supplement: Supplementary file 1 [file Old_Maths_Appendix.tex]

We develop our results in three parallel ways. First, in~\cref{app:Intuitive_Maths}, we study simple two source problems and pedagogically derive our results. Second, in ~\cref{sec:multivariate_representations}, we state the full inequality constraints, \cref{thm:linear_autoencoding}, and formally prove them using the same type of argument as in the pedagogical approach. Finally, in \cref{app:perturbative_approach}, we study the more general setting of invertible linear mixtures of sources and use a third, pertubative, approach to derive more general conditions under which a modular solution is optimal. These conditions recover our main inequalities as a special case. The three presentations of the result are independent, and readers may choose whichever they find more palatable. Then, in \cref{app:range_independent}, we prove the corollary \cref{thm:range_ind_corollary}. Finally, in \cref{app:ellipse_equivalence}, we show the equivalence between the two characterisations of the condition, via either the set of inequalities or the convex hull.

\subsection{Intuitive Development for Two Sources}\label{app:Intuitive_Maths}

\subsubsection{Problem Statement}

To begin, we study our simplest setting: a positive linear autoencoder that has to represent two bounded, scalar, mean-zero, sources, $x^{[i]}$ and $y^{[i]}$. These are encoded in a representation $\vz^{[i]}\in \mathbb{R}^N$, where $N$ is the number of neurons, which we will always assume to be as large as we need it to be, and in particular larger than the number of encoded variables. Our first constraint is given by the architecture. The representation is a linear function of the inputs plus a constant bias, and you must be able to decode the variables from the representation using an affine readout transformation:
\begin{equation}\label{eq:readin_readout_constraint}
\vz^{[i]} = \mW_{\text{in}}\begin{bmatrix}
        x^{[i]} \\ y^{[i]}
    \end{bmatrix} + \vb_{\text{in}} \qquad 
    \mW_{\text{out}} \cdot \vz^{[i]} + \vb_{\text{out}} = \begin{bmatrix}
        x^{[i]} \\ y^{[i]}
    \end{bmatrix}
\end{equation}
Where $\mW_{\text{in}}$ and $\vb_{\text{in}}$ are the readin weight matrix and bias, and $\mW_{\text{out}}$ and $\vb_{\text{out}}$ are the readout weight matrix and bias.

Our second constraint, inspired on the one hand by the non-negativity of biological neural firing rates, and on the other by the success of the ReLU activation function, is the requirement that the representation is non-negative: $\vz^{[i]} \geq {\bf 0}$. 

Subject to these constraints we optimise the representation to minimise an energy-use loss:
\begin{equation}\label{eq:total_loss}
    \mathcal{L} = \frac{1}{D}\sum_{i=1}^D ||\vz^{[i]}||^2 + \lambda (||\mW_{\text{out}}||^2_F + ||\mW_{\text{in}}||_F^2) = \langle||\vz^{[i]}||^2\rangle_i + \lambda (||\mW_{\text{out}}||^2_F + ||\mW_{\text{in}}||_F^2)
\end{equation}
This loss is inspired on the one hand by biology, in particular by the efficient coding hypothesis \citep{attneave1954some, barlow1961possible} and its descendants. These theories argue that neural firing should perform its functional role (e.g. encoding information) maximally energy-efficiently, for example by using the smallest firing rates possible, and has been used to understand neural responses across tasks, brain areas, individuals, and organisms \citep{laughlin2001energy, seenivasan2022efficient}. Our loss can be seen as a slight generalisation of this idea, by minimising energy use both through firing rates and through synapses \citep{harris2012synaptic}. On the other hand, this loss is similar to weight decay, a widely used regularisation technique in machine learning, that has long been linked to a simplicity bias in neural networks \citep{krogh1991simple}.

Our question can now be simply posed. What properties of the sources $x^{[i]}$ and $y^{[i]}$ ensure that they are optimally represented in disjoint sets of neurons? Equivalently, when does the representation modularise? The arguments of \citet{whittington2022disentanglement} can be used to show that if the two sources are statistically independent they should optimally modularise. We will find a much weaker set of conditions are necessary and sufficient for modularisation. In particular, we derive precise conditions on the range of allowed $(x,y)$ pairs that ensures modularising is optimal. For example, we will show that if the sources are range-symmetric ($|\min_i x^{[i]}| = \max_i x^{[i]}$) and extreme point independent, meaning $\min_i (x^{[i]} + y^{[i]}) = \min_i x^{[i]} + \min_i y^{[i]}$, they should modularise.

The structure of our argument goes as follows, by assumption the representation is a affine transformation of the inputs:
\begin{equation}\label{eq:linear_rep}
    \vz^{[i]} = \vu x^{[i]} + \vv y^{[i]} + \vb
\end{equation}
We will show that, for any fixed encoding sizes $||\vv||$ and $||\vu||$, the weight loss ($||\mW_{\text{out}}||_F^2 + ||\mW_{\text{in}}||_F^2$) is minimised by orthogonalising $\vv$ and $\vu$, in particular, by modularising the representation. We will then derive the conditions under which, for fixed encoding size, the activity loss is minimised by modularising the representation. If, whatever the encoding sizes, both losses are minimised by modularising, and the activity loss is minimised only by modularising (i.e. there are no other solutions that are equally good), the optimal representation is modular. Conversely, if the activity loss is not minimised by modularising, then you can always decrease the loss by slightly mixing the representation, hence the optimal representation is mixed.

\subsubsection{Conditions for Modularisation}

For simplicity we will make the following assumptions, that will be relaxed later:
\begin{enumerate}\label{list:assumptions}
    \item The sources are linearly uncorrelated, $\langle x^{[i]} y^{[i]} \rangle_i = \frac{1}{D} \sum_{i=1}^D x^{[i]} y^{[i]} = 0$
    \item The sources are range-symmetric around zero, i.e. $|\min_i x^{[i]}| = \max_i x^{[i]}$ and $|\min_i y^{[i]}| = \max_i y^{[i]}$
\end{enumerate}
We will consider the two losses in turn. 

\subsubsection{Weight Loss}\label{sec:weight_loss}


\begin{figure}[h]
    \centering
    \includegraphics[width=5in]{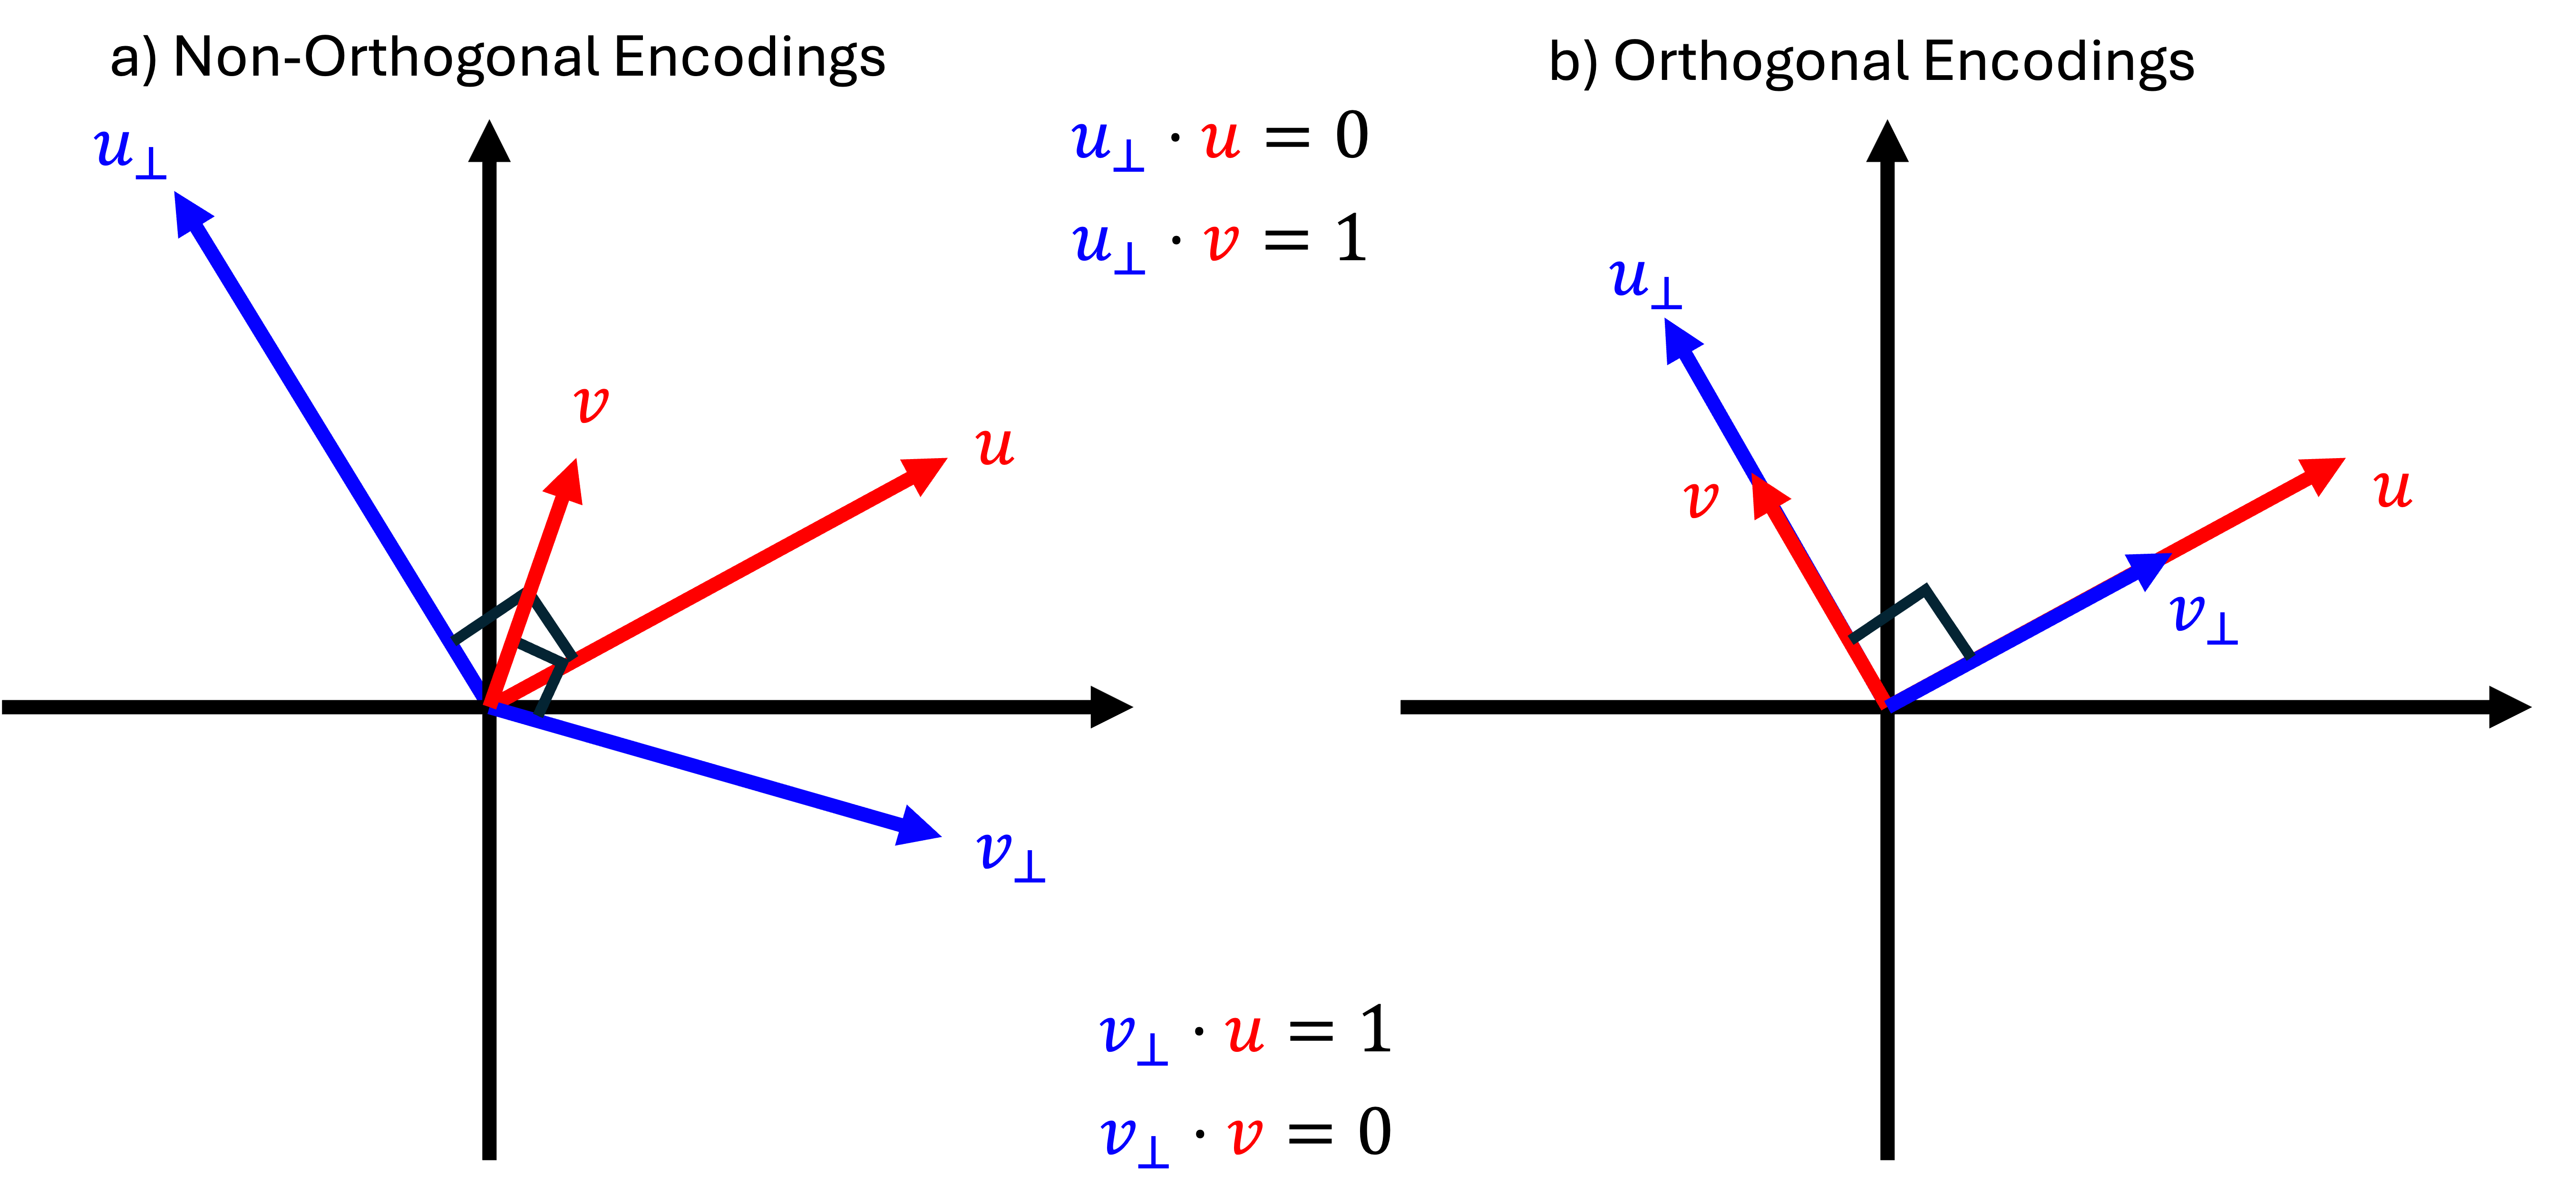}
    \caption{Schematics showing that modular representations minimise readout weight energy, $||W_{\text{out}}||_F^2$,  independent of encoding size. Aligning the encoding vectors (a) necessarily requires longer pseudoinverse vectors than an orthogonal solution (b), for example a modular solution.}
    \label{fig:weight_loss}
\end{figure}


First, for a given linear representation of the form in equation~\ref{eq:linear_rep}, the minimum squared norm readout matrix has the following form:
\begin{equation}
    \mW_{\text{out}} = \begin{bmatrix}
        \vv_\perp^T \\ \vu_\perp^T
    \end{bmatrix}
\end{equation}
Where $\vv\perp$ and $\vu_\perp$ are the two vectors in the span of $\vu$ and $\vv$ with the property that $\vv_\perp^T\vv = 0$ and $\vv_\perp^T\vu = 1$, and the equivalent conditions for $\vu_\perp$ (as in figure~\ref{fig:weight_loss}). To convince yourself of this consider the fact that these are the only two vectors in this plane that will produce the desired output, and you could add off-plane components to them, but that would only increase the weight loss for no gain, since:
\begin{equation}
    ||\mW_{\text{out}}||_F^2 = \Tr[\mW_{\text{out}}\mW_{\text{out}}^T] = ||\vu_\perp||^2 + ||\vv_\perp^2||
\end{equation}
These vectors, $\vv\perp$ and $\vu_\perp$, are the rows of the psuedoinverse, so henceforth we shall call these vectors the pseudoinverse vectors.

Then, with $\theta$ denoting the angle between $\vv$ and $\vu$, the readout loss can be developed using simple trigonometry:
\begin{equation}
    ||\mW_{\text{out}}||^2_F = ||\vv_\perp||^2  + ||\vu_\perp||^2 = \frac{1}{\sin^2(\theta)}\bigg(\frac{1}{||\vu||^2} + \frac{1}{||\vv||^2}\bigg)
\end{equation}
This has two interpretable properties. First, the larger the encoding the smaller the weight cost, and, second, the more aligned the two encodings the larger the weight cost. Both make a lot of sense, the more teasing apart of the representation is needed to extract the variable, the larger the weights, and the higher the loss. One claim we'll use later is that, for a given encoding size $||\vu||$ and $||\vv||$, all solutions with $\vu ^T \vv = 0$ are equally optimal. In particular, this is true of the modular solution:
\begin{equation}
    \vu = \begin{bmatrix}
        \vu' \\ {\bf 0}
    \end{bmatrix} \quad \vv = \begin{bmatrix}
        {\bf 0} \\ \vv'
    \end{bmatrix}
\end{equation}
Thus far we've discussed was the output weight cost. The input weight norm is even simpler:
\begin{equation}
    ||\mW_{\text{in}}||_F^2 = ||\begin{bmatrix}
        \vu & \vv
    \end{bmatrix}||_F^2 = \Tr[\mW_{\text{in}}^T\mW_{\text{in}}] = ||\vu||^2 + ||\vv^2||
\end{equation}
So, for a fixed encoding size, i.e. fixed $||\vu||^2$ and $||\vv||^2$, this loss is actually fixed. It therefore won't effect the optimal alignment of the representation.

Therefore we find, as advertised, that the weight loss is minimised by a modular solution.

\subsubsection{Activity Loss and Combination}

We now turn to the activity loss and study when it is minimised by modularising. We will play the following game. Let's say you have a non-modular, mixed, representation; i.e. a representation in which at least one neuron has mixed tuning to both $x$ and $y$:
\begin{equation}\label{eq:mixed_representation}
    z_n^{[i]} = u_n x^{[i]} + v_n y^{[i]} + \Delta_n
\end{equation}
Where, $\Delta_n = -\min_i [u_n x^{[i]} + v_n y^{[i]}]$ is the minimal bias required to make the representation non-negative. We will find the conditions under which, depending on the mixing coefficients ($u_n$ and $v_n$), you decrease the loss by forming the modular solution:
\begin{equation}\label{eq:modular_representation}
    \vz_n^{[i]} = \begin{bmatrix}
        u_n x^{[i]} \\ v_n y^{[i]}
    \end{bmatrix} - \begin{bmatrix}
        |u_n|  \min_i x^{[i]}\\ |v_n|  \min_i y^{[i]}
    \end{bmatrix} = \begin{bmatrix}
        u_n x^{[i]} \\ v_n y^{[i]}
    \end{bmatrix} + \begin{bmatrix}
        |u_n| b_x \\ |v_n| b_y
    \end{bmatrix}
\end{equation}
Where $b_x = - \min_i x^{[i]}$ is the bias required for a modular encoding of $x^{[i]}$. If, for a given $x^{[i]}$ and $y^{[i]}$, it is true that modularising decreases the loss for all mixings ($u_n$ and $v_n$) then the modular representation has the optimal energy loss. If there are conditions when modularising increases the loss, then you can always usefully demodularise the representation to decrease the activity loss, and we'll find that the optimal solution is not perfectly modular.

Let's analyse the activity loss of these two representations, for the modular representation (eq:~\ref{eq:modular_representation}):
\begin{equation}\label{eq:modular_activity_loss}
\langle||\vz^{[i]}_n||^2\rangle_i = u_n^2(\langle (x^{[i]})^2\rangle_i + b_x^2)) + v_n^2(\langle (y^{[i]})^2\rangle + b_y^2)
\end{equation}
And compare it to the mixed solution:
\begin{equation}\label{eq:demodularised_activity_loss}
    \langle(z^{[i]}_n)^2\rangle_i = u_n^2\langle (x^{[i]})^2\rangle_i + v_n^2\langle (y^{[i]})^2\rangle_i + \Delta_n^2
\end{equation}
Mixing is prefered over modularity, for a given $u_n$ and $v_n$, when:
\begin{equation}\label{eq:simple_mixing_inequality}
    (\min_i [u_n x^{[i]} + v_n y^{[i]}])^2 =\Delta_n^2 < u_n^2b_x^2 + v_n^2b_y^2 = u_n^2\min_i(x^{[i]})^2 + v_n^2\min_i(y^{[i]})^2
\end{equation}
Let's get some intuition for what this is saying. Take the simple setting when $v_n \approx 0$, i.e. we're considering a mixed neuron that mainly codes for $x$, with a little bit of $y$. Then two equivalent modular neurons are worse than this hypothetical mixed neuron if, to second order in $v_n$, $\Delta_n < |u_n|b_x + \frac{v_n^2 b_y^2}{|u_n|b_x}$. Since $\Delta_n$ is the mixed bias, this means that mixing a small amount of $y$ into the representation of $x$ is preferable when doing so effectively does not increase the required bias, relative to the bias for only encoding $x$ ($|u_n|b_x$). For this to be true $u_n x^{[i]}$ must have the same minima as $u_n x^{[i]} + v_n y^{[i]}$. For small enough $v_n$, an equivalent phrasing of this condition is that at the times at which $u_n x^{[i]}$ takes its minimal value, $y^{[i]}$ is non-negative. 

\begin{figure}[h]
    \centering
    \includegraphics[width=5in]{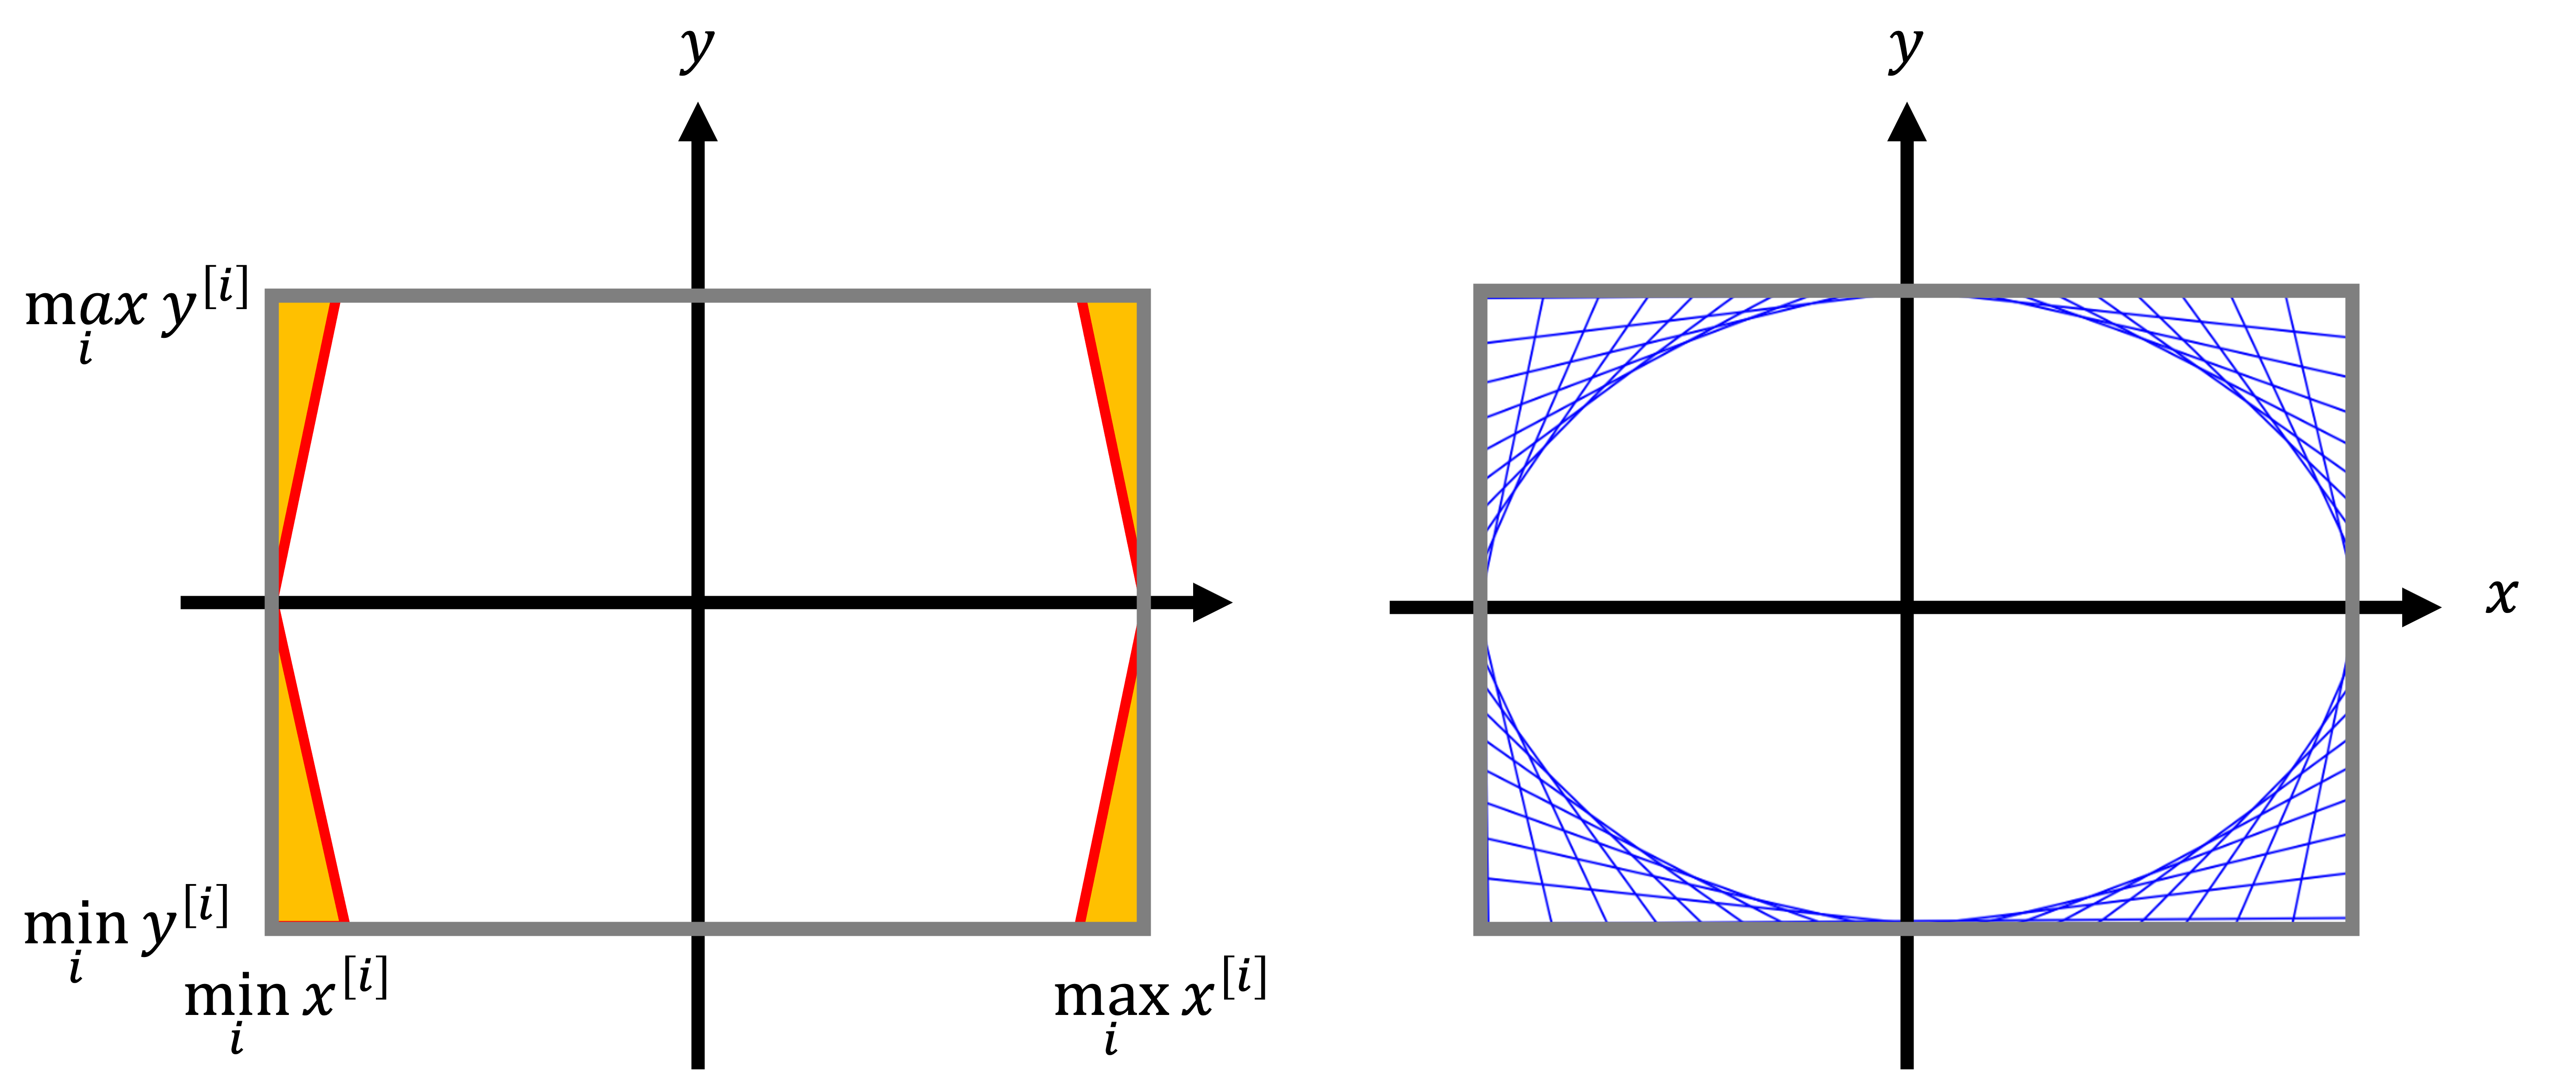}
    \caption{Visualising constraints via corner-cutting. Left: The optimal representation will prefer a mixture containing a small amount of $y$ over modularised if any of the orange shaded regions are missing from the co-range of $x$ and $y$. Right: Drawing these lines for all mixings creates a set of infinitely many lines, each corresponds to the data that must be missing for a particular mixed neuron to be preferable to the equivalent modular solution.}
    \label{fig:corner_cutting_intuition}
\end{figure}

We can visualise this conditions by plotting the allowed range of $x^{[i]}$ and $y^{[i]}$, \cref{fig:corner_cutting_intuition}. In grey is the bounding box given by the minima and maxima of $x$ and $y$.  Assume for now that $u_n$ and $v_n$ are positive. For a fixed small value of $v_n$ the minima of $u_n x^{[i]} + v_ny^{[i]}$ remains $u_n\min_i x^{[i]}$ if there are no datapoints below the line $u_n \min_i x^{[i]} = u_n x + v_n y$. Drawing this onto the square, this means there are no datapoints below the red line, in the bottom-left orange region. If this condition is met the representation should mix because this mixed neuron (given by the particular $u_n$ and $v_n$ ratio) is better than an equivalent modular solution. 

That was for positive $u_n$ and $v_n$. If either of them are negative then you draw a different line corresponding to that sign combination, e.g.: $u_n \min_i x^{[i]} = |u_n| x - |v_n|y$. This produces the top-left red line and orange area, again, if there are no datapoints in this shaded region a mixed neuron with mixture coefficients, $|u_n|$ and $-|v_n|$ is better than the equivalent modular solution. Repeating this for the other sign combinations fills in the other four corners. Hence, we find that a mixed solution in which a small amount of $y$ is mixed into a neuron encoding $x$ is better when there are no datapoints in at least one of the four corner regions. 

That was for one particular pair of $u_n$ and $v_n$, this hypothetical mixed neuron that encodes mainly $x$ with a pinch of $y$. But to be optimal the modular solution has to be better than all possible mixed neurons. As such we get a family of such constraints: for each mixing of the sources we get a different inequality on the required bias, as described by equation~\ref{eq:simple_mixing_inequality}. Each of these can be similarly visualised as a corner missing from the co-range of $x$ and $y$, the blue lines in \cref{fig:corner_cutting_intuition} right. If any one of these corners is missing from the co-range of $(x,y)$ then the mixed solution is better, else the modular solution is preferred. We can already see the shape of the ellipse emerging that will be the basis of our later version of the theorem, see \cref{app:ellipse_equivalence}.

\subsubsection{Combining two Analyses}

We studied the two loss terms separately, how do they interact?

If the inequality conditions, \cref{eq:simple_mixing_inequality}, are satisfied, then the activity loss prefers a modular solution over all mixed representations with the same fixed encodings sizes, $||\vv||$ and $||\vu||$. Further, the weight loss is also minimised, for a fixed encoding size, by modularising. Therefore the optimal solution will be modular.

Conversely, if one of the inequalities is broken then the activity loss is not minimised at the modular solution. We can move towards the optimal mixed solution by creating a new mixed encoding neuron with infinitesimally low activity, and mixed in proportions given by the broken inequality. This neuron can be created by taking small pieces of the modular encoding of each source, in proportion to the mixing. Doing this will decrease the activity loss. Further, the weight loss is minimised at the modular solution, so, to first order, moving away from modular solution doesn't change it. Therefore, for each modular representation, we have found a mixed solution that is better, so the optimal solution is not modular. Therefore, if one of the inequalities is broken, the optimal representation will be mixed.

\subsubsection{Relaxing Assumptions}

We now show how the modularisation behaviour of variables that break the two assumptions listed in~\ref{list:assumptions} can be similarly understood. 

\paragraph{Correlated Variables}\label{sec:correlated_variables}

Correlated variables are easy to deal with, they simply introduce an extra term into the difference in activity losses, equation~\ref{eq:demodularised_activity_loss} minus equation~\ref{eq:modular_activity_loss}:
\begin{equation}\label{eq:correlated_demodularised_activity_loss}
    \langle||\vz^{[i]}_n||^2\rangle_i - \langle(z^{[i]}_n)^2\rangle_i= u_n^2b_x^2 + v_n^2b_y^2 - 2u_nv_n\langle x^{[i]}y^{[i]}\rangle_i - \Delta_n^2
\end{equation}
This leads to a slightly updated inequality, the solution mixes if:
\begin{equation}\label{eq:bound_inequality}
    \Delta_n < \sqrt{u_n^2b_x^2 + v_n^2b_y^2 - 2v_nu_n\langle x^{[i]} y^{[i]}\rangle_i}
\end{equation}

\begin{figure}[h]
    \centering
    \includegraphics[width=5in]{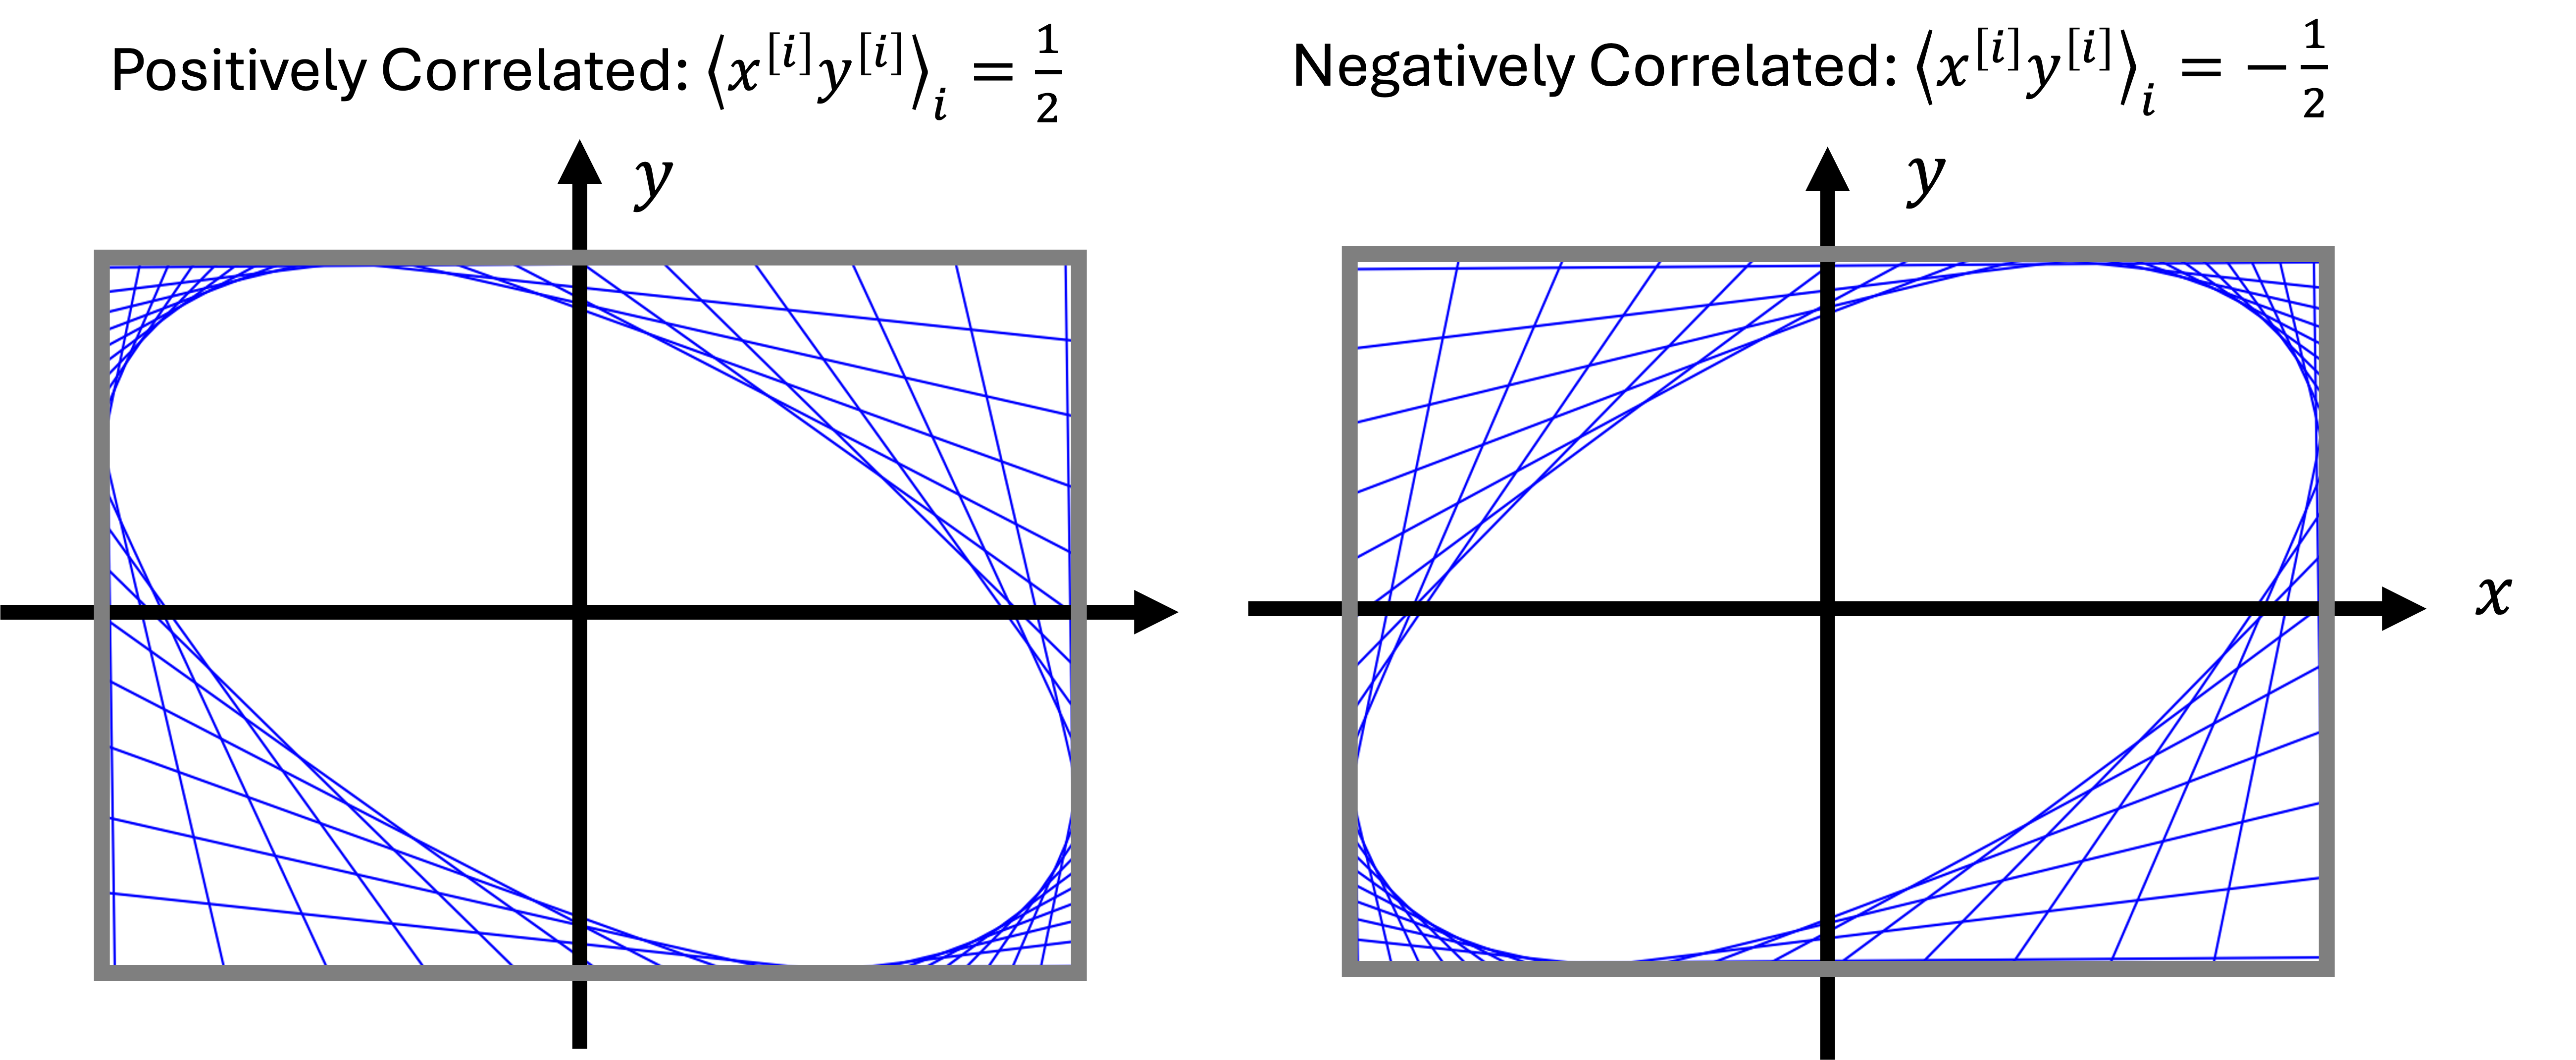}
    \caption{Visualising how correlations change corner-cutting. Left: It is energetically costly to align the encodings of positively correlated variables}
    \label{fig:correlated_corner_cutting}
\end{figure}
The effect of this change is to shift the corner-cutting lines that determine whether a modular or mixed solution is optimal. This can be understood intuitively. If the variables are positively correlated then positively aligning their representations is energetically costly, and negatively aligning them is energy saving. This is most simply seen in one line of maths. The energy cost contains the following term:
\begin{equation}
    \langle (\vu x^{[i]} + \vv y^{[i]})^2\rangle_i = ||\vu||^2\langle(x^{[i]})^2\rangle_i + ||\vv||^2\langle(y^{[i]})^2\rangle_i + \vu^T\vv \langle x^{[i]}y^{[i]}\rangle_i
\end{equation}
So if the correlation is positive, $\vu^T\vv$ should be negative to decrease the energy, i.e. the encodings should be anti-aligned. Hence, correlated variables have a preferred orientation.

Similarly, the corner cutting has an associated `direction of alignment'. If the bottom left corner is missing that means that building a neuron whose representation is a mix of positively aligned $x$ and $y$ is preferable, as it has a smaller minima, requiring less bias. Similarly, if the bottom right corner is missing, the representation can take advantage of that by building neurons that encode $x$ negatively and $y$ positively, i.e. anti-aligning them. 

If these two directions, one from the correlations and one from the range-dependent positivity effects, agree, then it is `easier' to de-modularise, i.e. less of a corner needs to be missing from the range to de-modularise. Conversely, if they mis-align it is harder. This is why the correlations shift the corner-cutting lines up or down depending on the corner. We can see this in~\cref{fig:correlated_corner_cutting}. When the variables are positively correlated it becomes `easier' to mix in the anti-aligned corners, at bottom-right or top-left, and harder at the aligned pair, while the converse is true of the negatively correlated example.

Of interest is a result we can find that guarantees modularisation regardless of the correlation. For these bounded variables the covariances, $\langle x^{[i]}y^{[i]}\rangle_i$, are themselves bounded. The most postively co-varying two variables can be is to be equal, then the covariance becomes the variance. Further, the bounded, symmetric, mean-zero variable with the highest variance spends half its time at its max, and half at its min. Similar arguments but with a minus sign for the most anti-covarying representations tell us that:
\begin{equation}\label{eq:extreme_covar}
    -b_y b_x \leq \langle x^{[i]} y^{[i]}\rangle_i \leq b_x b_y
\end{equation}
These results are similar to those in \citet{hossjer2022sharp}. Putting this into~\cref{eq:bound_inequality}, the maximal bounding bias for the most positively or negatively correlated variables to prefer modularising:
\begin{equation}\label{eq:corr_extreme_ineq_1}
    \Delta_n > |u_n| b_x + |v_n| b_y
\end{equation}
This bound is the development of equation~\ref{eq:bound_inequality} in two cases. First in the maximally positively correlated case when the sign of $u_i$ and $v_i$ are opposite. Second in the maximally negatively correlated case where the coefficient signs are the same.

From this we can derive the following interesting result, the pedagogical version of~\cref{thm:linear_autoencoding_app}. We will say that if, across the dataset, when $x^{[i]}$ takes its maximum (or minimum) value, $y^{[i]}$ takes both its maximum and minimum values for different datapoints, the two variables are extreme point independent. Another way of saying this is that there is non-zero probability of each of the corners of the rectangle. Now, no matter the value of the correlation, extreme point independence variables should modularise. This is because:
\begin{equation}
    \Delta_n = -\min_i\bigg[u_n x^{[i]} + v_n y^{[i]} \bigg] = -|u_n|\min_i x^{[i]} - |v_n|\min_i y^{[i]} = |u_n|b_x + |v_n|b_y 
\end{equation}
Hence, we find that even the loosest inequality possible, equation~\ref{eq:corr_extreme_ineq_1}, is never satisfied. Further, since the variables are extreme point independent their covariance never achieves the equalities in equation~\ref{eq:extreme_covar}, so inequality~\ref{eq:corr_extreme_ineq_1} is not satisfied and the variables should modularise.

This means that symmetric extreme point independent variables should always modularise, regardless of how correlated they are. Conversely, for variables that are not quite extreme point independent (perhaps they are missing some corner), there is always a value of their correlation that would de-modularise them.

\paragraph{Range Asymmetric Variables}\label{sec:range_assymmetry}

Thus far we have assumed $|\min_i x^{[i]}| = \max_i x^{[i]}$, for simplicity. This is not necessary. If this is not the case than there is a `direction' the variable wants to be encoded. Consider encoding a single variable either positively ($z_+^{[i]} = |u|x^{[i]} + b$) or negatively ($z_-(t) = -|u|x^{[i]} + b$), the losses will differ:
\begin{equation}
    \langle (z_+^{[i]})^2\rangle_i = |u|^2 \big(\langle (x^{[i]})^2\rangle_i + (\min_i x^{[i]})^2\big) \qquad \langle (z_-^{[i]})^2\rangle_i = |u|^2 \big(\langle (x^{[i]})^2\rangle_i + (\max_i x^{[i]})^2\big)
\end{equation}
This is simply expressing the fact that if a variable is mean-zero but asymmetrically bounded then more of the data must be bunched on the smaller side, and you should choose the encoding where most of this data stays close to the origin.

Now, assume without loss of generality that for each variable $b_x = |\min_t x(t)| \leq \max_t x(t)$. Then the identical argument to before carries through for the modularisation behaviour around the lower left corner. Around the other corners however, things are more complicated. There might be a corner missing from the lower right quadrant, but to exploit it you would have to build a mixed neuron that is positively tuned to $y$ but negatively tuned to $x$. This would incur a cost, as suddenly the $x$ variable is oriented in its non-optimal direction. Therefore the calculation changes, because the modular solution can always choose to `correctly' orient variables, so doesn't have to pay this cost. This is all expressed in the same inequalities, eqn.~\ref{eq:bound_inequality}:
\begin{equation}
    \Delta_n < \sqrt{u_n^2b_x^2 + v_n^2b_y^2 - 2v_nu_n\langle x^{[i]} y^{[i]}\rangle_i}
\end{equation}

%Then, following the same logic as before, to modularise:
%\begin{equation}
%\begin{split}
%   \Delta_i < 
%|u_i|x_{\max} + |v_i|b_y - \sqrt{u_i^2x_{\max}^2 + v_i^2b_y^2 - 2v_iu_i\langle x(t) y(t)\rangle_t - u_i^2(x_{\max}^2 - b_x^2)}\\

%|u_i|x_{\max} + |v_i|b_y - \sqrt{u_i^2b_{x}^2 + v_i^2b_y^2 - 2v_iu_i\langle x(t) y(t)\rangle_t} = |u_i|(x_{\max}-b_x) + \Delta_c
%\end{split}
%\end{equation}
%Where we have denoted the previous critical value of $\Delta_i$ with $\Delta_c$ (i.e. the right hand side of equation~\ref{eq:bound_inequality}). You can see that the $x$ flipping cost has the effect of increasing the critical $\Delta_i$ by $|u_i|(x_{\max}-b_x)$, i.e. mixing the encodings must be more co-operative than previously to pay this cost.

%This was for the bottom right corner, if you want to work out how much $\Delta$ must be in order to de-modularise via the top right corner you have to add both $|u_i|(x_{\max}-b_x)$ and $|v_i|(y_{\max}-b_y)$, i.e. the flipping costs of both $x$ and $y$.

This effect can also be viewed in the required range plots, where it translates to a much larger corner being cut off in order to pay the cost of switching around the variables, \cref{fig:Asymetric_Range_Corner_Cutting}.

\begin{figure}[h]
    \centering
    \includegraphics[width=3in]{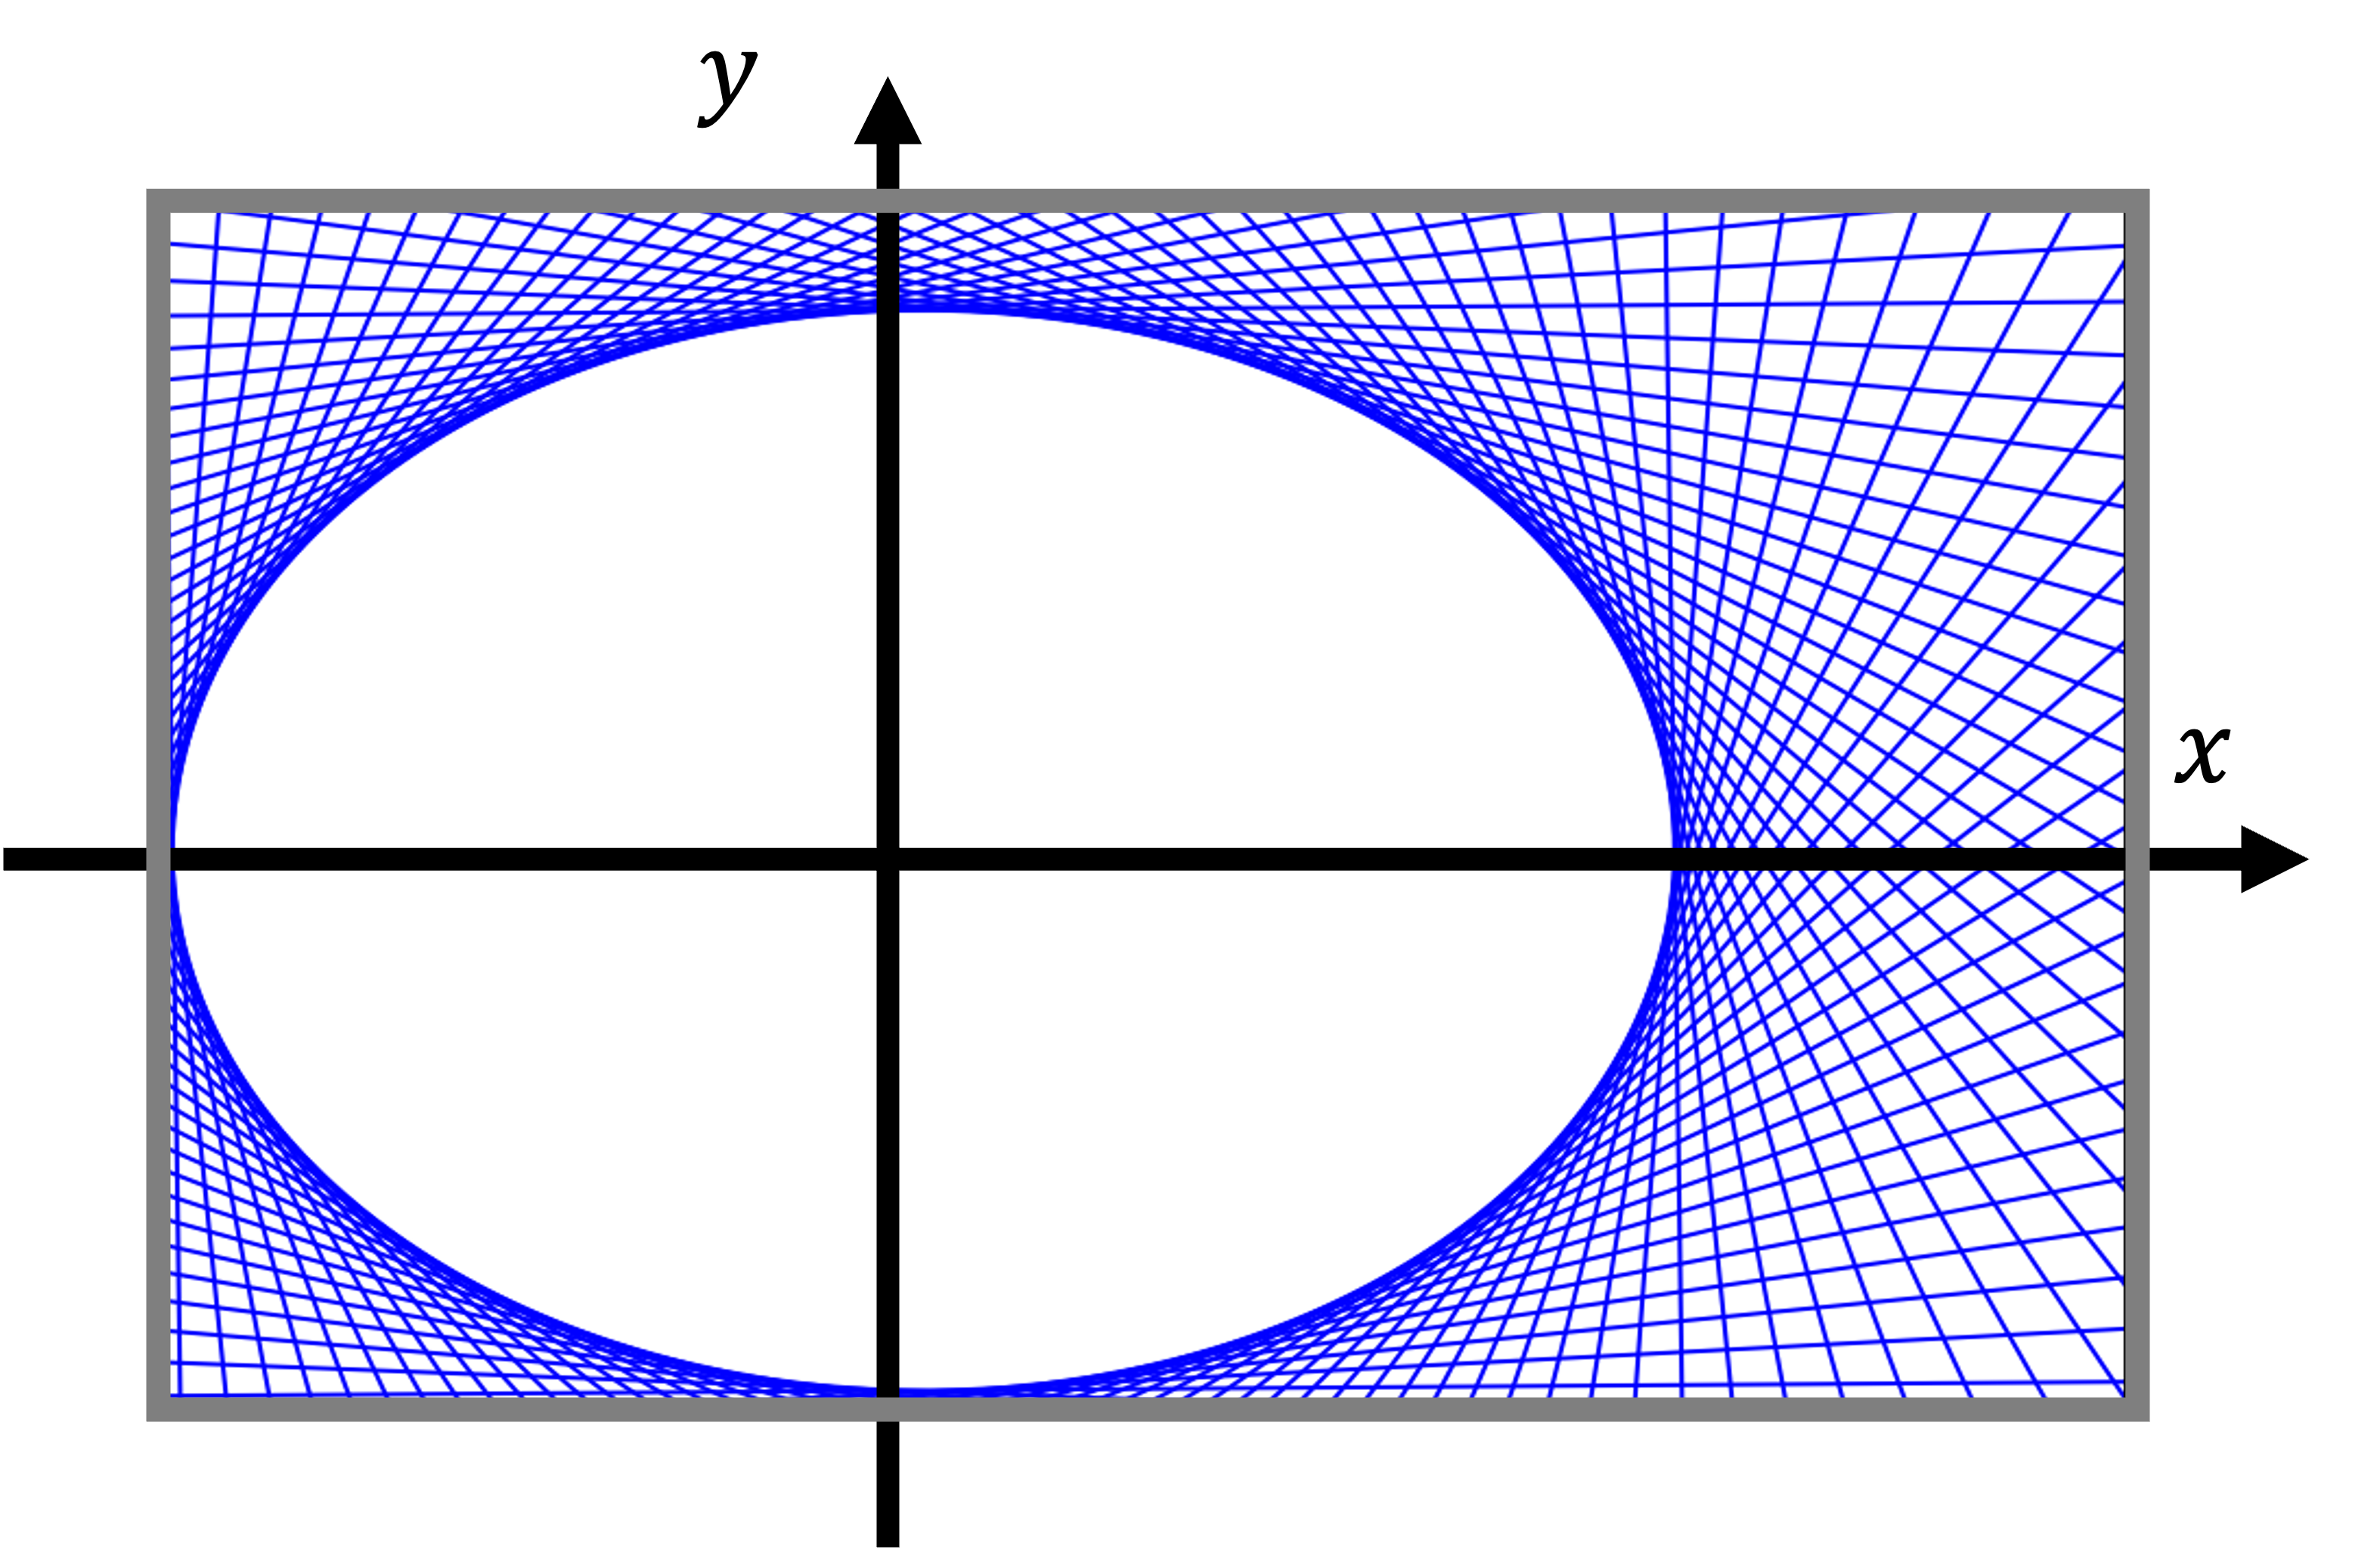}
    \caption{Visualising how asymmetric ranges change corner-cutting. When the ranges are asymmetric much larger corners must be cut off the `longer' sides before mixing becomes preferable to modularising.}
    \label{fig:Asymetric_Range_Corner_Cutting}
\end{figure}

%One quick point is that, for range assymetric variables, the covariance is unbounded, and so it can be large enough to demodularise any pair of variables. Assume for demonstration you have two variables with the same max and min ($b_{\max}$ and $b_{\min}$). The highest covariance you can reach with this pair of bounded, mean-zero, variables is for both variables to spend most of their time either both at the top of their range with some probability $p$, or at the bottom with some probability $1-p$. Because the variables are mean-zero $b_{\max}p = -b_{\min}(1-p)$. Now the covariance is $b_{\min}^2\frac{1-p}{p}$, which can grow to any value, and demodularise anything. 

\paragraph{Remaining Assumptions}

There are two remaining assumptions about the variables, that they are mean-zero and that they are bounded. Neither of these are really assumptions. The first since we don't penalise biases in the weight losses you can add or remove a constant from the variables for no cost. That means adding or removing the mean from the variables doesn't change the problem, so our results generalise to non-mean-zero variables, but all the conditions apply to the mean-subtracted versions of the variables. The second boundedness constraint appears more fundamental, but for any finite dataset the variables will have a maximum and minimum value. These values will be the important ones that determine modularisation.

\subsection{Full Theoretical Treatment}\label{sec:multivariate_representations}

Now we shall prove our main result in generality.

\begin{theorem}[Main Result]\label{thm:linear_autoencoding_app} 
    Let $\vs \in \mathbb{R}^{d_s}$, $\vz \in \mathbb{R}^{d_z}$, $\mW_{\mathrm{in}} \in\mathbb{R}^{d_z\times d_s}$, $\vb_{\mathrm{in}}\in\mathbb{R}^{d_z}$, $\mW_{\mathrm{out}}\in\mathbb{R}^{d_s\times d_z}$, and $\vb_{\mathrm{out}}\in\mathbb{R}^{d_s}$, with $d_z > d_s$. Consider the constrained optimization problem
    \begin{equation}
        \begin{aligned}
        \min_{\mW_\mathrm{in}, \vb_\mathrm{in}, \mW_\mathrm{out}, \vb_\mathrm{out}}& \quad
            \left\langle ||\vz^{[i]}||_2^2\right\rangle_i + \lambda\left(||\mW_{\mathrm{out}}||_F^2 + ||\mW_{\mathrm{in}}||_F^2\right) \\
        \text{\emph{s.t. }}& \quad \vz^{[i]} = \mW_{\mathrm{in}} \vs^{[i]} + \vb_{\mathrm{in}}, \; \vs^{[i]} =  \mW_{\mathrm{out}} \vz^{[i]} + \vb_{\mathrm{out}}, \; \vz^{[i]} \geq 0,
        \end{aligned}
    \end{equation}
    where $i$ indexes samples of $\vs$.
    At the minima of this problem, each row of $\mW_{\mathrm{in}}$ has at most one non-zero entry, i.e. the representation modularises, iff the following inequality is satisfied for all $\vw \in \mathbb{R}^{d_s}$:
    \begin{equation}\label{eq:linear_ae_inequality_app}
         \left(\min_i [\vw^\top \vs^{[i]}]\right)^2 + \sum^{d_s}_{j,j'\neq j}w_{j}w_{j'}\left\langle \bar{s}^{[i]}_j \bar{s}^{[i]}_{j'} \right\rangle_i 
         >
         \sum_{j=1}^{d_s} \left(w_j \min_i\bar{s}^{[i]}_j\right)^2,
    \end{equation}
    where $\bar{\vs} := \vs -\left\langle \vs^{[i]}\right\rangle_{i}$ and assuming that 
    $\left|\min_i\bar{s}^{[i]}_j\right| \leq \max_i\bar{s}^{[i]}_j \; \forall j \in [d_s]$ w.l.o.g.
\end{theorem}

To show this statement we begin by showing a lemma: that, for a fixed encoding size, the weight loss is minimised by orthogonalising the encoding of each source, the multidimensional analogue of~\cref{sec:weight_loss}. Writing the representation as an affine function of the de-meaned sources:
\begin{equation}
    \vz^{[i]} = \sum_{j=1}^{d_s} \vu_j s_j^{[i]}+ \vb  = \sum_{j=1}^{d_s} \vu_j (s_j^{[i]} - \langle s_j^{[k]}\rangle_k)+ \vb' = \sum_{j=1}^{d_s} \vu_j \bar{s}_j^{[i]} + \vb'
\end{equation}
then by fixed encoding size we mean that each $|\vu_j|$ is fixed. We express things in terms of mean-zero variables $\bar{s}_j^{[i]}$ since it is easier and we can freely shift by a constant offset.

\begin{theorem}[Modularising Minimises Weight Loss]\label{thm:weight_loss_minimised_by_modularising} The weight loss, $||\mW_{\mathrm{out}}||_F^2 + ||\mW_{\mathrm{in}}||_F^2$, is minimised, for fixed encoding magnitudes, $|\vu_j|$, by modularising the representation. 

\end{theorem}

\begin{proof}
    First, we know that $\mW_{\text{in}}$ must be of the following form:
    \begin{equation}
        \mW_{\text{in}} = \begin{bmatrix}
            \vu_1 & \hdots & \vu_{d_s}
        \end{bmatrix}
    \end{equation}
    And therefore for a fixed encoding size the input weight loss is constant:
    \begin{equation}
        ||\mW_{\text{in}}||_F^2 = \Tr[\mW_{\text{in}}^T\mW_{\text{in}}] = \sum_{j=1}^{d_s} |\vu_j|^2
    \end{equation}
    So let's study the output weights, these are defined by the way they map the representation back to the sources:
    \begin{equation}
        \mW_{\text{out}}\cdot \vz^{[i]} + \vb_{\text{out}} = \begin{bmatrix}
            s_1^{[i]} \\ \vdots \\ s_{d_s}^{[i]}
        \end{bmatrix}
    \end{equation}

The min-norm $\mW_{\text{out}}$ with this property is the Moore-Penrose Pseudoinverse, i.e. the matrix:
\begin{equation}
    \mW_{\text{out}} = \begin{bmatrix}
        \mU_1^T\\ \vdots \\ \mU_{d_s}^T
    \end{bmatrix}
\end{equation}
Where each pseudoinverse $\mU_i$ is defined by $\mU_i^T\vu_j = \delta_{ij}$ and lying completely within the span of the encoding vectors $\{\vu_j\}$. We can calculate the norm of this matrix:
\begin{equation}
    |\mW_{\text{out}}|_F^2 = \Tr[\mW_{\text{out}}\mW_{\text{out}}^T] = \sum_{j=1}^{d_s} |\mU_j|^2
\end{equation}
Now, each of these capitalised pseudoinverse vectors must have some component along its corresponding lower case vector, and some component orthogonal to that:
\begin{equation}
    \mU_j = \frac{1}{|\vu_j|^2}\vu_j + \vu_{j,\perp}
\end{equation}
We've chosen the size of the component along $\vu_j$ such that $\mU_j^T\vu_j = 1$, and the $\vu_{j,\perp}$ is chosen so that $\mU_j^T\vu_k = \delta_{jk}$. Now, for a fixed size of $|\vu_j|$, this sets a lower bound on the size of the weight matrix:
\begin{equation}
    |\mW_{\text{out}}|_F^2 = \sum_{j=1}^{d_s} \frac{1}{|\vu_j|^2} + |\vu_{j,\perp}|^2 \geq  \sum_{j=1}^{d_s} \frac{1}{|\vu_j|^2}
\end{equation}
And this lower bound is achieved whenever the $\{\vu_j\}_{j=1}^{d_s}$ vectors are orthogonal to one another, since then $\vu_{j,\perp} = 0$. Therefore, we see that, for a fixed size of encoding, the weight loss is minimised when the encoding vectors are orthogonal, and that is achieved when the code is modular. 
\end{proof}

Now we will turn to studying the activity loss, and find conditions under which a modular representation is better than a mixed one. We compare two representations, a mixed neuron:
\begin{equation}
    z_n^{[i]} = \sum_{j=1}^{d_s} u_{nj}\bar{s}_j^{[i]} + \Delta_n = \sum_{j=1}^{d_s} u_{nj}\bar{s}_j^{[i]} - \min_i[\sum_{j=1}^{d_s} u_{nj}\bar{s}_j^{[i]}]
\end{equation}
And another representation in which we break this neuron apart into its modular form, preserving the encoding size of each source:
\begin{equation}
    \vz_n^{[i]} = \begin{bmatrix}u_{n1}\bar{s}_1^{[i]} \\ \vdots \\ u_{nd_{s}}\bar{s}_{d_s}^{[i]} \end{bmatrix} - \begin{bmatrix}|u_{n1}|\min_j \bar{s}_{1}^{[j]} \\ \vdots \\ |u_{nd_{s}}|\min_j\bar{s}_{d_s}^{[i]}\end{bmatrix}
\end{equation}
The activity loss difference between the modular and mixed representations is:
\begin{equation}
     \sum_{j}u_{nj}^2 (\min_i\bar{s}_{j}^{[i]})^2 - (\min_i[\sum_{j=1}^{d_s} u_{nj}\bar{s}_j^{[i]}])^2 - \sum_{j=1,k\neq j}^{d_s} u_{nj}u_{nk}\langle\bar{s}_j^{[i]}\bar{s}_k^{[i]}\rangle_{i}
\end{equation}
So the modular loss is smaller if, for all $\vu_n \in\mathbb{R}^{d_s}$:
\begin{equation}\label{eq:key_inequality}
    (\min_i[\sum_{j=1}^{d_s} u_{nj}\bar{s}_j^{[i]}])^2
    > \sum_ju_{nj}^2(\min_i\bar{s}_{j}^{[i]})^2 - \sum_{j,k\neq j}u_{nj}u_{nk}\langle\bar{s}_j^{[i]}\bar{s}_k^{[i]}\rangle_{i}
\end{equation}
Further, we can see that if this equation holds for one vector, $\vu$, it also holds for any scaled version of that vector, therefore we can equivalently require the inequality to be true only for unit norm vectors.

So, if these inequalities are satisfied, both the weight and activity loss are minimised at fixed encoding size by modularising, and this holds for all encoding sizes, therefore the optimal solution must be modular. Hence these conditions are sufficient for modular solutions to be optimal.

Conversely, if one of the inequalities is broken then the activity loss is not minimised at the modular solution. We can move towards the optimal mixed solution by creating a new mixed encoding neuron with infinitesimally low activity, and mixed in proportions given by the broken inequality. This neuron can be created by taking small pieces of the modular encoding of each source, in proportion to the mixing. Doing this will decrease the activity loss. Further, the weight loss is minimised at the modular solution, so, to first order, moving away from modular solution doesn't change it. Therefore, for each modular representation, we have found a mixed solution that is better, so the optimal solution is not modular. 

\subsection{Range-Independent Variables}\label{app:range_independent}

We will now prove this corollary, that was pedagogically discussed in \cref{app:Intuitive_Maths}:

\begin{corollary}
    In the same setting as~\cref{thm:linear_autoencoding} the optimal representation modularises if all sources are pairwise extreme-point independent, i.e. if
    \begin{equation}
        \min_i \bigg[s_j^{[i]} \bigg| s^{[i]}_{j'} \in \left\{\max_{i'} s^{[i']}_{j'}, \min_{i'} s^{[i']}_{j'}\right\}\bigg] = \min_i s_j^{[i]}
    \end{equation}
    for all $j,j' \in [d_s]^2$.
\end{corollary}

\begin{proof}
If the variables are extreme-point independent then we can take the min inside the sum in the definition of the mixed neuron bias:
\begin{equation}
z_n^{[i]} = \sum_{j=1}^{d_s} u_{nj}\bar{s}_j^{[i]} + \Delta_n = \sum_{j=1}^{d_s} u_{nj}\bar{s}_j^{[i]} - \min_i[\sum_{j=1}^{d_s} u_{nj}\bar{s}_j^{[i]}] = \sum_{j=1}^{d_s}\bigg( u_{nj}\bar{s}_j^{[i]} - \min_i[u_{nj}\bar{s}_j^{[i]}]\bigg)
\end{equation}

Now we can compute the activity loss:
\begin{equation}
\begin{aligned}
    \langle (z_n^{[i]})^2\rangle_i =  \\
 \sum_{j=1}^{d_s}\langle\bigg( u_{nj}\bar{s}_j^{[i]} - \min_i[u_{nj}\bar{s}_j^{[i]}]\bigg)^2\rangle_i + \sum_{j,j'=1, j\neq j}^{d_s}\langle \bigg( u_{nj}\bar{s}_j^{[i]} - \min_i[u_{nj}\bar{s}_j^{[i]}]\bigg)\bigg( u_{nj}\bar{s}_{j'}^{[i]} - \min_i[u_{nj}\bar{s}_{j'}^{[i]}]\bigg)\rangle_i
\end{aligned}
\end{equation}
The cross terms at the end are strictly positive, and each of the squared terms on the left is the same or larger than its corresponding modular neuron, since either $u_{nj}$ is positive and it is the same, or $u_{nj}$ is negative and it is greater than or equal to the equivalent modular neuron. Therefore the mixed energy cost is larger than the modular energy cost for extreme-point independent variables.
\end{proof}

\begin{comment}
\newpage

\begin{corollary}
    In the same setting as~\cref{thm:linear_autoencoding}, if $\left|\min_i\bar{s}^{[i]}_j\right| = \max_i\bar{s}^{[i]}_j \; \forall j \in [d_s]$, i.e. each source is range-symmetric, then the optimal representation modularises if all sources are pairwise extreme-point independent, i.e. if
    \begin{equation}
        \min_i \bigg[s_j^{[i]} \bigg| s^{[i]}_{j'} \in \left\{\max_{i'} s^{[i']}_{j'}, \min_{i'} s^{[i']}_{j'}\right\}\bigg] = \min_i s_j^{[i]}
    \end{equation}
    for all $j,j' \in [d_s]^2$.
\end{corollary}

\begin{proof}
    
If sources are range-symmetric and mean-zero then the largest their variance can be is  $(\max_i s_j^{[i]})^2$, which occurs when the source takes its maximum and minimum values each with probability $\frac{1}{2}$ \citep{hossjer2022sharp}. Further, by Cauchy-Schwarz, the covariance between two variables is bounded by their variances, so we get a bound. Further, while two variables are maximally correlated if they are equal, they are maximally anticorrelated if one is minus the other. Hence the covariance is bounded from below by the same quantity with a minus sign. Putting these together: 
\begin{equation}
    -\max_i s_j^{[i]} \max_i s_k^{[i]}< \langle s_j^{[i]}s_k^{[i]}\rangle_i < \max_i s_j^{[i]} \max_i s_k^{[i]}
\end{equation}
Create the following vector:
\begin{equation}
    \vm = \begin{bmatrix}
        \max_i s_1^{[i]} \\\max_i s_2^{[i]} \\ \vdots \\ \max_i s_{d_s}^{[i]}
    \end{bmatrix}
\end{equation}
Then, using the bounds on the covariances, we derive that:

\begin{equation}\label{eq:inequality_bound}
         \sum_{j=1}^{d_s} \left(w_j \min_i\bar{s}^{[i]}_j\right)^2 - \sum^{d_s}_{j,j'\neq j}w_{j}w_{j'}\left\langle \bar{s}^{[i]}_j \bar{s}^{[i]}_{j'} \right\rangle_i < (\vw^T\vm)^2
 \end{equation}
Now we just return to the final term in the original inequality. For extreme-point indepedent variables this simplifies considerable:
\begin{equation}
    (\min_i [\vw^\top \vs^{[i]}])^2 = (\vw^T\min_i \vs^{[i]})^2 = (\vw^T\vm)^2
\end{equation}
Therefore, the inequalities become:
\begin{equation}
    (\min_i [\vw^\top \vs^{[i]}])^2 = (\vw^T\vm)^2 > 
         \sum_{j=1}^{d_s} \left(w_j \min_i\bar{s}^{[i]}_j\right)^2 - \sum^{d_s}_{j,j'\neq j}w_{j}w_{j'}\left\langle \bar{s}^{[i]}_j \bar{s}^{[i]}_{j'} \right\rangle_i
\end{equation}
Which we can see, using \cref{eq:inequality_bound}, is now true for all $\vw$, therefore the representation should be modular, regardless of the correlations.
\end{proof}
\end{comment}

\subsection{Perturbative Approaches to Modularisation of Linearly Mixed Sources}\label{app:perturbative_approach}

Now we consider a more general setting than that stated in the main paper. We allow the input data, $\vx^{[i]}$, to be a linear mixture of the sources: $\vx^{[i]} = \mA\vs^{[i]}$. We then similarly ask when should the optimal nonnegative, linear, efficient, representation be modular? We derive a more general exact condition for modularisation that recovers our main result as a special case.

\begin{theorem}\label{thm:linearly_mixed_sources} 
    Let $\vs \in \mathbb{R}^{d_s}$, $\vx \in\mathbb{R}^{d_x}$, $\vz \in \mathbb{R}^{d_z}$, $\mW_{\mathrm{in}} \in\mathbb{R}^{d_z\times d_x}$, $\vb_{\mathrm{in}}\in\mathbb{R}^{d_x}$, $\mW_{\mathrm{out}}\in\mathbb{R}^{d_x\times d_z}$, $\vb_{\mathrm{out}}\in\mathbb{R}^{d_x}$, and $\mA\in\mathbb{R}^{d_x\times d_s}$ with $d_z > d_s$ and $d_x \geq d_s$, and $\mA$ is rank $d_s$. Consider the constrained optimization problem
    \begin{equation}
        \begin{aligned}
        \min_{\mW_\mathrm{in}, \vb_\mathrm{in}, \mW_\mathrm{out}, \vb_\mathrm{out}}& \quad
            \left\langle ||\vz^{[i]}||_2^2\right\rangle_i + \lambda\left(||\mW_{\mathrm{in}}||_F^2 + ||\mW_{\mathrm{out}}||_F^2\right) \\
        \text{\emph{s.t. }}& \quad \vz^{[i]} = \mW_{\mathrm{in}} \vx^{[i]} + \vb_{\mathrm{in}}, \; \vx^{[i]} =  \mW_{\mathrm{out}} \vz^{[i]} + \vb_{\mathrm{out}}, \; \vz^{[i]} \geq 0,
        \end{aligned}
    \end{equation}
    where $i$ indexes a finite set of samples of $\vs$, and $\vx^{[i]} = \mA\vs^{[i]}$. The optimal representation is modular, i.e. one in which each latent, $z_j^{[i]}$, is a function of a single source, iff the following inequality is satisfied for all $\vw \in \mathbb{R}^{d_s}$:
    \begin{equation}\label{eq:linearly_mixed_inequalities}
         \langle(\vw^T\vs^{[i]})^2\rangle_i + (\min_i \vw^T\vs^{[i]})^2 + \lambda\vw^T(\mA^T\mA)^{-1}\vw > \lambda \vw^T\mD^{-2}(\mA^T\mA)\mD^{-2}\vw
    \end{equation}
    where $\bar{\vs} := \vs -\left\langle \vs^{[i]}\right\rangle_{i}$, assuming that 
    $\left|\min_i\bar{s}^{[i]}_j\right| \leq \max_i\bar{s}^{[i]}_j \; \forall j \in [d_s]$ w.l.o.g., and where
    $\mD$ is a diagonal matrix with diagonal elements:
    \begin{equation}
        D_{jj} = \sqrt[4]{\frac{\lambda ((\mA^T\mA)_{jj})^2}{\langle (s_j^{[i]})^2\rangle_i + (\min_i s_j^{[i]})^2 + \lambda ((\mA^T\mA)^{-1})_{jj}}}
    \end{equation}
\end{theorem}

Using the method as for the original statement, this too can be turned into an visually easier claim about the convex hull and bounding a particular set:

\begin{theorem}\label{thm:linearly_mixed_sources_convex_hull} 
    In the same setting as \cref{thm:linearly_mixed_sources} form the matrix $\mS$:
    \begin{equation}
        \mS = \lambda\mD^{-2}(\mA^T\mA)\mD^{-2} - \lambda(\mA^T\mA)^{-1} -\langle \vs^{[i]}(\vs^{[i]})^T\rangle_i
    \end{equation}
    then an equivalent condition to \cref{eq:linearly_mixed_inequalities} is that the convex hull of the datapoints encloses the set $E = \{\vy: \vy^T\mS^{-1}\vy = 1\}$.
\end{theorem}

We cannot attack this with the same techniques as before, as, unless the columns of $\mA$ are orthogonal, the weight loss is no longer minimised by modularising. We therefore take a different approach, we study the linear stability of the optimal modular solution and show that iff the inequalities in theorem \cref{thm:linearly_mixed_sources} are satisfied the optimal modular solution is a local minima. We then additionally prove that the loss can be phrased as a convex optimisation problem and use that to tell us that local minima are global minima.

\begin{figure}[h]
    \centering
    \includegraphics[width=5.5in]{Figures/Linear_Mixing.png}
    \caption{We linear mix range-independent data through some matrix $A$ and consider the optimisation problem for two different values of $\lambda$. In one case (top row) the matrix $\mS$ is positive definite, meaning $E$ is an ellipse, and the convex hull encloses it. Thus, theory predicts that the representation should modularise and the empirics match this. Yet, (bottom row), increasing $\lambda$ by a small amount makes the matrix $\mS$ indefinite, and $E$ becomes a parabola that no finite dataset can enclose in its convex hull. Thus we get a mixed optimal representation.}
    \label{fig:Linear_Mixing}
\end{figure}

\subsubsection{Optimal Modular Solution}

First we need to find the optimal modular solution. This can be implemented by $d_S$ neurons (since the loss is rotationally invariant adding more neurons makes no difference). Let's write this solution as:
\begin{equation}
    \vz_M^{[i]} = \sum_{j=1}^{d_S}d_j(s_j^{[i]}-\min_i s_j^{[i]})\ve_j = \sum_{j=1}^{d_S}d_j \bar{s}_j^{[i]}\ve_j
\end{equation}
Where $\ve_j$ are the canonical basis vectors, $d_j$ represents the strength of the encoding of each source, and the subscript M denotes the fact it is modular. Stacking the $d_j$ elements into a diagonal matrix $\mD$ we can derive each of the three loss terms. We know that:
\begin{equation}
     \vz^{[i]} = \mW_{\text{in}}\vx^{[i]} + \vb_{\text{in}} = \mW_{\text{in}}\mA\vs^{[i]} + \vb_{\text{in}} = \mD\vs^{[i]} + \vb_{\text{in}} 
\end{equation}
Hence:
\begin{equation}
    \mW_{\text{in}} = \mD\mA^\dagger \qquad \mW_{\text{out}} = \mW_{\text{in}}^\dagger = \mA\mD^{-1}
\end{equation}
where $\dagger$ denotes the pseudoinverse. Hence:
\begin{equation}
    ||\mW_{\text{in}}||_F^2 = \Tr[\mW_{\text{in}}^T\mW_{\text{in}}] = \Tr[\mD^2\mA^\dagger(\mA^\dagger)^T] = \Tr[\mD^2\mO_A^{-1}]
\end{equation}
\begin{equation}
    ||\mW_{\text{out}}||_F^2 = \Tr[\mD^{-2}\mO_A]  
\end{equation}
Where we've defined $\mO_A = \mA^T\mA$, and then $\mA^\dagger(\mA^\dagger)^T = \mO_A^{-1}$, as can be seen using the SVD of $\mA$ and $\mA^\dagger$.

Denote with $\alpha_j^2$ the diagonal elements of $\mO_A$, they represent how strongly a particular source is encoded in the data. Further, denote with $(\alpha'_j)^2$ the diagonal elements of $\mO^{-1}_A$, these represent the lengths of the `pseudoinverse vectors' in \cref{fig:weight_loss}. If the encodings of each source are orthogonal they are just the inverse of the encoding sizes, $\alpha_j$, if not, they also tell you how `entangled' a source's representation is. In the limit of colinearity of sources, $\alpha'_j$ go to infinity representing the fact that the modular solution cannot exist. In terms of these variables we can write the whole loss as:
\begin{equation}
    \mathcal{L} = \sum_{j=1}^{d_s} d_j^2[\langle (s_j^{[i]})^2\rangle_i + (\min_i s_j^{[i]})^2 + \lambda (\alpha'_j)^2] + \frac{\lambda \alpha^2_j}{d_j^2}
\end{equation}
Then the optimal choice of encoding sizes is:
\begin{equation}
    (d_j^*)^4 = \frac{\lambda \alpha_j^2}{\langle (s_j^{[i]})^2\rangle_i + (\min_i s_j^{[i]})^2 + \lambda (\alpha'_j)^2}
\end{equation}

\subsubsection{Perturbing the Optimal Modular Solution}

Now let's add the following perturbation to the optimal representation:
\begin{equation}
    \vz^{[i]} = \sum_{j=1}^{d_s}(d_j^* - \delta_j)(s_j^{[i]}-\min_i s_j^{[i]})\ve_j + \ve_{d_s+1}(\vw^T\vs^{[i]} - \min_i \vw^T\vs^{[i]})
\end{equation}
This represents an arbitrary perturbation to the modular solution combined with adding a new mixed neuron with mixing $\vw$. We could add more mixed neurons, but to the order we consider they contribute independently, allowing you to consider them one-by-one. We will assume all the $\delta_j$ and $\vw$ are small, and expand the loss to second order in them. If this perturbation decreases the loss for any $\vw$ then the optimal representation is mixed, else the optimal modular solution is a local minima. First let's create some new matrices:
\begin{equation}
    \tilde{\mD} = \begin{bmatrix}
        d_1^* - \delta_1 & 0 & \hdots & 0\\
        0 & d_2^* - \delta_2 & \hdots & 0\\
        \vdots & \vdots & \ddots & \vdots \\
        0 & 0 & \hdots & d_{d_s}^* - \delta_{d_S} \\
        0 & 0 & \hdots & 0
    \end{bmatrix}
    \qquad     \mE = \begin{bmatrix}
        0 & 0 & \hdots & 0\\
        0 & 0 & \hdots & 0\\
        \vdots & \vdots & \ddots & \vdots \\
        0 & 0 & \hdots & 0 \\
        w_1 & w_2 & \hdots & w_{d_s}
    \end{bmatrix}
\end{equation}
Then I claim the min-norm $\mW_{\text{in}}$ and $\mW_{\text{out}}$ are given by:
\begin{equation}
    \mW_{\text{in}} = (\tilde{\mD} + \mE)\mA^\dagger \qquad \mW_{\text{out}} = \mA(\tilde{\mD} + \mE)^\dagger
\end{equation}
These are the min-norm solutions, because they are pseudoinverses and they're min-rank, i.e. rank $d_s$. The form of the losses will again be things like:
\begin{equation}
    ||\mW_{\text{in}}||_F^2 = \Tr[ (\tilde{\mD} + \mE)^T(\tilde{\mD} + \mE)\mO_A^{-1}] = \Tr[ \mO_D\mO_A^{-1}] \qquad ||\mW_{\text{out}}||_F^2 = \Tr[\mO_D^{-1}\mO_A]
\end{equation}
We can see the following:
\begin{equation}
    \mO_D = (\tilde{\mD} + \mE)^T(\tilde{\mD} + \mE) = \tilde{\mD}^2 + \vw\vw^T
\end{equation}
Then, using Sherman-Morrison:
\begin{equation}
    \mO_D^{-1} = \tilde{\mD}^{-2} -\frac{\tilde{\mD}^{-2}\vw\vw^T\tilde{\mD}^{-2}}{1 + \vw^T\tilde{\mD}^{-2}\vw}
\end{equation}
We're only going to be working to second order, so we can simplify this expression significantly:
\begin{equation}
    \mO_D^{-1} = \tilde{\mD}^{-2} -\mD^{-2}\vw\vw^T\mD^{-2} + \mathcal{O}(\delta^3)
\end{equation}
Now it is a bit of algebra to derive the three losses:
\begin{equation}
    ||\mW_{\text{in}}||_F^2 = \Tr[\mD^2\mO_A^{-1}] - 2\Tr[\text{diag}(d^*_j\delta_j)\mO_A^{-1}] + \Tr[\text{diag}(\delta_j^2)\mO^{-1}_A] + \vw^T\mO_A^{-1}\vw
\end{equation}
\begin{equation}
    ||\mW_{\text{out}}||_F^2 = \Tr[\mD^{-2}\mO_A] + 2\Tr[\text{diag}(\frac{\delta_j}{(d^*_j)^3})\mO_A] + \Tr[\text{diag}(\frac{\delta_j^2}{(d^*_j)^4})\mO_A] - \vw^T\mD^{-2}\mO_A\mD^{-2}\vw
\end{equation}
\begin{equation}
    \langle ||\vz^{[i]}||^2\rangle_i = \sum_{j=1}^{d_s}
    (\langle (s_j^{[i]})^2\rangle_i + (\min_i s_j^{[i]})^2)((d^*_j)^2 - 2d^*_j\delta_j+\delta_j^2) + \langle(\vw^T\vs^{[i]})^2\rangle_i + (\min_i \vw^T\vs^{[i]})^2
\end{equation}
There are first order terms in $\delta_j$, but you can check that at the optimal modular solution these are 0. Then we have to consider the second order terms, there are some proportional to $\delta_j^2$:
\begin{equation}
    \sum_{j=1}^M \delta_j^2(\lambda (\alpha_j')^2 + \frac{3\lambda \alpha_j^2}{(d_j^*)^4} + \langle (s_j^{[i]})^2\rangle_i + (\min_i s_j^{[i]})^2)
\end{equation}
But, you will notice that this term is always positive! Therefore, it always increases the loss, so we might as well set $\delta_j = 0$, and move on to the only term that might cause mixing to be optimal, if this term is positive then modular solutions are locally the best!
\begin{equation}\label{eq:linearly_mixed_inequalities_II}
     \langle(\vw^T\vs^{[i]})^2\rangle_i + (\min_i \vw^T\vs^{[i]})^2 + \lambda\vw^T\mO_A^{-1}\vw - \lambda \vw^T\mD^{-2}\mO_A\mD^{-2}\vw > 0
\end{equation}
This is the linearly mixed equivalent of our inequality, and proves the original statement, \cref{thm:linearly_mixed_sources}.

\subsubsection{Re-deriving Original Result}

As a corollary we can rederive our main result, \cref{thm:linear_autoencoding}. To do this we assume $\vx^{[i]} = \vs^{[i]}$. This occurs when $\mA = I$, $\mO_A = \mO^{-1}_A = I$; then:
\begin{equation}
    (d_j^*)^4 = \frac{\lambda}{\lambda + \langle (s_j^{[i]})^2\rangle_i + (\min_i s_j^{[i]})^2} \qquad (d_j^*)^{-4} = 1 + \frac{1}{\lambda}(\langle (s_j^{[i]})^2\rangle_i + (\min_i s_j^{[i]})^2)
\end{equation}
Then you can rewrite \cref{eq:linearly_mixed_inequalities_II} as:
\begin{equation}
\begin{split}
     \langle(\vw^T\vs^{[i]})^2\rangle_i + (\min_i \vw^T\vs^{[i]})^2 + \lambda\vw^T\vw - \lambda \vw^T\mD^{-4}\vw =\\ \langle(\vw^T\vs^{[i]})^2\rangle_i + (\min_i \vw^T\vs^{[i]})^2 - \sum_{j=1}^M w_j^2 (\langle (s_j^{[i]})^2\rangle_i + (\min_i s_j^{[i]})^2) > 0
 \end{split}
\end{equation}
Which exactly recovers the previous inequalities!

This shows that, when these inequality conditions are met, the best modular solution is a local optima. In the next section we show that the problem is convex, and hence this local optima is a global optima.

\subsection{Problem is Convex}

In this section we are going to rewrite the problem to show it is convex. Inspired by \citep{sengupta2018manifold} we're going to write the entire optimisation problem in terms of the representational similarity matrix. Create the full hidden layer representation matrix, $\mZ \in \mathbb{R}^{d_z \times K}$ where $K$ is the total number of datapoints, then the representational similarity is $\mD = \mZ^T\mZ \in \mathbb{R}^{K \times K}$. In order to show the problem is convex with respect to this variable we need to first show that the feasible set of allowed $\mD$ matrices is a convex set, and second show that the objective function is a convex function of $\mD$. We will do each of these in turn.

\subsubsection{Convex Feasible Set}

The representation has to obey three constraints:
\begin{itemize}
    \item It has to be positive $\mZ \geq {\bf 0}$
    \item It has to be an affine function of the inputs. Let's create a source matrix $\mS \in \mathbb{R}^{d_s \times K}$. Now $\mZ = \mW_{\text{in}}\mS + \vb_{\text{in}}$. To write this more concisely let's define:
    \begin{equation}
        \mS' = \begin{bmatrix}
            \mS \\
            {\bf 1}
        \end{bmatrix} \qquad \mW_{\text{in}}' = \begin{bmatrix}
            \mW_{\text{in}} & \vb_{\text{in}}
        \end{bmatrix} \quad \text{such that} \quad \mZ = \mW'_{\text{in}}\mS'
    \end{equation}
    \item An affine map has to relate the representation back to the inputs, using analagously defined variables this is: $\mS = \mW_{\text{out}}'\mZ'$. If the input matrix, $\mW_{\text{in}}'$, has full column rank, such a readout affine map will always exist.
\end{itemize}

We will now show that the set of dot product matrix of a representation $\mZ$ that satisfies each of these constraints form a convex set, and since the intersection of many convex sets forms a convex set \citep{boyd2004convex}, the set of feasible dot product matrices that satisfy all three criteria will be convex. 

To begin with the easiest (having read \citep{sengupta2018manifold}), the set of dot product matrices with unconstrained ranks formed from vectors that are themselves all positive ($\mD = \mZ^T\mZ$ for $\mZ \geq 0$) form a convex set called the set of completely positive matrices \citep{berman2003completely}.

The second constraint is the affine input constraint. Take two dot product matrices formed from representations that are affine functions of their input: $\mD = \mZ^T\mZ$, $\mZ = \mW_{\text{in}}'\mS'$, and $\tilde{\mD} = \tilde{\mZ}^{T'}\tilde{\mZ}$, $\tilde{\mZ} = \tilde{\mW}_{\text{in}}'\mS'$. Take their convex combination:
\begin{equation}
    \lambda\mD + (1-\lambda)\tilde{\mD} = \mS^{'T}(\lambda\mW_{\text{in}}^{'T}\mW_{\text{in}}' + (1+\lambda)\tilde{\mW}_{\text{in}}^{'T}\tilde{\mW}_{\text{in}}')\mS' \quad \lambda \in [0, 1]
\end{equation}
Since $d_z > d_s$ and each input matrix must have full column rank, both $\mW_{\text{in}}^{'T}\mW_{\text{in}}'$ and $\tilde{\mW}_{\text{in}}^{'T}\tilde{\mW}_{\text{in}}'$ are full rank positive definite matrices, therefore their convex combination will be as well. Further any positive definite matrix can be decomposed into two parts, therefore we can write $\lambda\mW_{\text{in}}^{'T}\mW_{\text{in}}' + (1+\lambda)\tilde{\mW}_{\text{in}}^{'T}\tilde{\mW}_{\text{in}}' = \hat{\mW}_{\text{in}}^{'T}\hat{\mW}_{\text{in}}^{'}$ for some matrix $\hat{\mW}_{\text{in}}'$. Hence
\begin{equation}
    \lambda\mD + (1-\lambda)\tilde{\mD} = \mS^{'T}\hat{\mW}_{\text{in}}^{'T}\hat{\mW}_{\text{in}}^{'}\mS' = (\hat{\mW}_{\text{in}}^{'}\mS')^T(\hat{\mW}_{\text{in}}^{'}\mS') = \hat{\mZ}^T\hat{\mZ}
\end{equation}
And hence the convex combination of two dot product matrices of full-column rank affine functions of the input data will also be such a dot product matrix.

Finally, the representation can be used to perfectly reconstruct the inputs using an affine map if it is made from a readin matrix with full column rank. As in the paragraph above, the set of dot product matrices of representations formed from full column rank input matrices is a convex set, so too is the set of dot product matrices of affine decodable representations.

As all three sets are convex, we find that the set of feasible dot product matrices is a convex set.

\subsubsection{Convex Objective}

We will now rewrite the objective in terms of this dot product matrix, and show it is a convex function of the representational dot product matrix.

{\bf Activity} Begin with the activity loss:
\begin{equation}
    \langle ||\vz^{[i]}||_2^2\rangle_i = \frac{1}{K}\Tr[\mZ^T\mZ] = \frac{1}{K}\Tr[\mD]
\end{equation}
which since it is a linear function of $\mD$ is clearly a convex function.

{\bf Readin Weights} Next let's move to the readin weight loss. We know that $\mZ = \mW_{\text{in}}\mS + \vb_{\text{in}}{\bf 1}^T$. Given a set of sources and a representation, lets choose the min-norm mapping matrix using the pseudoinverse of the source matrix:
\begin{equation}
    \mW_{\text{in}} = (\mZ - \vb_{\text{in}}{\bf 1}^T)\mS^\dagger
\end{equation}
Then its frobenius norm is:
\begin{equation}
    ||\mW_{\text{in}}||_F^2 = \Tr[\mW_{\text{in}}^T\mW_{\text{in}}] = \Tr[\mS^\dagger\mS^{T,\dagger}(\mZ - \vb_{\text{in}}{\bf 1}^T)^T(\mZ - \vb_{\text{in}}{\bf 1}^T)] 
    \end{equation}
\begin{equation} 
    = \Tr[\mS^\dagger\mS^{T,\dagger}\mZ^T\mZ] -2{\bf 1}^T\mS^\dagger\mS^{T,\dagger}\mZ^T\vb_{\text{in}} + {\bf 1}^T\mS^\dagger\mS^{T,\dagger}{\bf 1}|\vb_{\text{in}}|^2
\end{equation}
Since each source is mean-zero $\mS{\bf 1} = {\bf 0}$. This means {\bf 1} is orthogonal to each of the rows of $\mS$. Since the columns of $\mS^\dagger$ and the rows of $\mS$ span the same space we derive that ${\bf 1}^T\mS^\dagger = {\bf 0}$, and so all but one of the terms above disappears, telling us that:
\begin{equation}
    ||\mW_{\text{in}}||_F^2 =\Tr[\mS^\dagger\mS^{T,\dagger}\mZ^T\mZ] = \Tr[\mS^\dagger\mS^{T,\dagger}\mD]
\end{equation}
This is also a linear function of $\mD$, so is again convex.

{\bf Readout Weights} Finally let's turn to the readout weights: $\mS = \mW_{\text{out}}\mZ + \vb_{\text{out}}{\bf 1}^T$. Given a representation, $\mZ$, we can derive the optimal bias choice using KKT conditions on the following lagrangian:
\begin{equation}
    ||\mW_{\text{out}}||_F^2 + \Tr[\Lambda^T(\mW_{\text{out}}\mZ + \vb_{\text{out}}{\bf 1}^T - \mS)]
\end{equation}
Where $\Lambda$ are lagrange multipliers that enforce the exact fitting of the data. The KKT conditions on this Lagrangian tell us that:
\begin{equation}
    \Lambda{\bf 1} = 0 \quad \mW_{\text{out}} = -\frac{1}{2}\Lambda\mZ^T \quad \mS = \mW_{\text{out}}\mZ + \vb_{\text{out}}{\bf 1}^T
\end{equation}
Combining these we can derive that:
\begin{equation}
    \vb_{out}{\bf 1}^T = \mS + \frac{1}{2}\Lambda\mZ^T\mZ
\end{equation}
Now we're going to right multiply by $(\mZ^T\mZ)^\dagger{\bf 1}$. Since ${\bf 1}\in\mathbb{R}^K$ is definitely in the span of the columns of $\mZ^T\mZ$, we know that $\mZ^T\mZ(\mZ^T\mZ)^\dagger{\bf 1} = {\bf 1}$, and hence the final term will be zero due the fixed point condition that $\Lambda{\bf 1} = 0$. Hence:
\begin{equation}\label{eq:b_out_defn}
    \vb_{\text{out}} = \frac{\mS\mZ^\dagger (\mZ^\dagger)^T\mathbf{1}}{||(\mZ^\dagger)^T\mathbf{1}||_2^2}
\end{equation}
Similarly to the above, the min-norm readout weights will be: $(\mS - \vb_{\text{out}}{\bf 1}^T)\mZ^\dagger$. Now we can study our readout weight loss:
\begin{equation}
    ||\mW_{\text{out}}||_F^2 = \Tr[(\mS - \vb_{\text{out}}{\bf 1}^T)^T(\mS - \vb_{\text{out}}{\bf 1}^T)\mZ^\dagger\mZ^{\dagger,T}]
\end{equation}
One can derive the following very useful fact by inserting the derived form of $\vb_{\text{out}}$ \cref{eq:b_out_defn} into the following equation:
\begin{equation}
    (\mS - \vb_{\text{out}}{\bf 1}^T)\mZ^\dagger\mZ^{\dagger,T}{\bf 1} = {\bf 0}
\end{equation}
Which is basically saying that when you use the optimal bias you don't waste precious readout weight energy fitting the mean shift of the data. Now we can see that all the cross terms in the readout weight loss will cancel and we're left with just:
\begin{equation}
     ||\mW_{\text{out}}||_F^2 = \Tr[\mS^T\mS\mZ^\dagger\mZ^{\dagger,T}]
\end{equation}
Using the SVD it is clear that $\mZ^\dagger\mZ^{\dagger,T} = \mD^{-1}$, hence our loss is:
\begin{equation}
    = \Tr[\mS^T\mS\mD^{-1}]
\end{equation}
Finally it's just left to show that this is a convex function of $\mD$. We can adapt Robert Israel's proof techique from stack exchange to show this setting is convex \url{https://math.stackexchange.com/questions/297635/is-the-trace-of-inverse-matrix-convex}. A twice differentiable function $f$ on an open subset $\mathbb{U}$ of a vector space $\mathbb{V}$ is convex iff:
\begin{equation}
    \frac{d^2}{dt^2} f(u + tv)|_{t=0} \geq 0 \quad \forall \quad u \in \mathbb{U}, v \in \mathbb{V}. 
\end{equation}
Adapting that to our setting we need to show that:
\begin{equation}
    \frac{d^2}{dt^2} \Tr(\mS^T\mS(\mD + t\mQ)^{-1})|_{t=0} \geq 0 \quad \forall \quad \mD \in \mathcal{S}^{KN_A}_+, \mQ \in \mathcal{S}^{KN_A} 
\end{equation}
Where $\mathcal{S}^{KN_A}$ denotes the set of symmetric $KN_A\times KN_A$ matrices, and $\mathcal{S}^{KN_A}_+$ is the set of positive definite symmetric matrices. By taylor expanding (A version of the Woodbury matrix lemma says that $(\mA - \mB)^{-1} = \sum_{k=0}^\infty (\mA^{-1}\mB)^k\mA^{-1}$), or otherwise, you can find that:
\begin{equation}
    \frac{d^2}{dt^2} \Tr(\mS^T\mS(\mD + t\mQ)^{-1})|_{t=0} = 2\Tr(\mS^T\mS\mD^{-1}\mQ\mD^{-1}\mQ\mD^{-1})
\end{equation}
Since $\mS^T\mS$ is symmetric and positive definite, we can rewrite this by defining $\mC = (\mS^T\mS)^\frac{1}{2}\mD^{-1}\mQ$, as $\Tr(\mC\mD^{-1}\mC^T)$. Since $\mD$ is positive definite (and therefore so too is $\mD^{-1}$), so is $\mC\mD^{-1}\mC^T$ and the trace is greater than or equal to zero. Hence the term is convex. 

So we have a convex function of a convex set, and therefore the whole problem is convex, there is a single globally optimal representational similarity matrix, $\mD^*$. If we find an optimal representation, $\mZ^*$, such that $\mZ^{*T}\mZ^* = \mD^*$, then all optimal representations will be related to it by an orthogonal transform that preserves the positivity of the representation, $\mZ^{*'} = \mU\mZ^*$. If an optimal representation is modular all orthogonal transforms that preserve positivity will be as well, so we derive that if a modular solution is a local optima, the global optima is modular.

\subsection{Equivalence of Convex Hull Formulation}\label{app:ellipse_equivalence}

In this section we prove \cref{thm:ellipse_equivalence}, an equivalent formulation of the infinitely many inequalities in \cref{thm:linear_autoencoding} in terms of the convex hull, restated below:

\begin{theorem}\label{thm:ellipse_equivalence_appendix} 
    In the setting as \cref{thm:linear_autoencoding}, define the following matrix:
    \begin{equation}
            \mS = \begin{bmatrix}
        (\min_i s_1^{[i]})^2 & -\langle s_1^{[i]} s_2^{[i]}\rangle_i & \hdots \\
        -\langle s_1^{[i]} s_2^{[i]}\rangle_i & (\min_i s_2^{[i]})^2 & \hdots \\
        \vdots & \vdots & \ddots
    \end{bmatrix}
    \end{equation}
    Define the set $E = \{\vy: \vy^T\mS^{-1}\vy = 1\}$. Then an equivalent statement of the modularisation inequalities \cref{eq:linear_ae_inequality}, is the representation modularises iff $E$ lies within the convex hull of the datapoints.  
\end{theorem}

Notice that the matrix $\mS$ is not even guaranteed to be positive semi-definite, meaning $E$ is not necessarily an ellipse. In these cases no convex hull can contain the unbounded quadric it forms, and the optimal solution is mixed regardless of the particular distribution of the datapoints.

We'll begin by rewriting the inequalities, then we'll show each direction of the equivalence.

\subsubsection{Rewrite Inequality Constraints}

The current form of the inequality is that, $\forall \vw \in \mathbb{R}^n$:
\begin{equation}
        (\min_i \vw^T\vs^{[i]})^2 + \sum_{j,j'\neq j}^{d_s} w_j w_{j'}\langle s_j^{[i]}s_{j'}^{[i]}\rangle_i \geq \sum_j w_j^2 (\min_i s_j^{[i]})^2
\end{equation}
If this equation holds for one vector, $\vw$, it also holds for all positively scaled versions of the vector, $\vv = \lambda\vw$ for $\lambda > 0$, so we can equivalently state that this condition must only hold for unit vectors, $\{\vw\in\mathbb{R}^n : |\vw|= 1\}$.

Construct the following matrix that depends on the correlations and the dimension-wise minima:
\begin{equation}
    \mS = \begin{bmatrix}
        (\min_i s_1^{[i]})^2 & -\langle s_1^{[i]} s_2^{[i]}\rangle_i & \hdots \\
        -\langle s_1^{[i]} s_2^{[i]}\rangle_i & (\min_i s_2^{[i]})^2 & \hdots \\
        \vdots & \vdots & \ddots
    \end{bmatrix}
\end{equation}
Then this condition can be rewritten:
\begin{equation}\label{eqn:min_inequality}
    (\min_i \vw^T\vs^{[i]})^2 \geq \vw^T\mS\vw\quad \forall \vw\in\mathbb{R}^n, |\vw| = 1
\end{equation}
Further, notice that we can swap the minima in the inequality for a maxima. We can do this because if the inequality is satisfied for a particular value of $\vw$ then the following inequality is satisfied for $-\vw$:
\begin{equation}\label{eqn:max_inequality}
    (\max_i \vw^T\vs^{[i]})^2 \geq \vw^T\mS\vw \quad \forall \vw\in\mathbb{R}^n, |\vw| = 1
\end{equation}
Since \cref{eqn:min_inequality} is satisfied for all $\vw$, and all $\vw$ have their $-\vw$ unit vector pairs, so is \cref{eqn:max_inequality}. Similarly, if \cref{eqn:max_inequality} is satisfied for all unit vectors $\vw$, \cref{eqn:min_inequality} is satisfied but using $-\vw$. Hence the two are equivalent. 

\subsubsection{Sufficiency of Condition}

First, let's show the convex hull enclosing $E$ is a sufficient condition. Choose an arbitrary unit vector $\vw$. Choose the point within $E$ that maximises the dot product with $\vw$:
\begin{equation}
    \vy_w = \argmax_{\vy\in E}\vw^T\vy 
\end{equation}
We can find $\vy_w$ by lagrange optimisation under the constraint that $\vy^T\mS^{-1}\vy = 1$:
\begin{equation}\label{eq:lagrange_ellipse}
    \vy_w = \frac{\mS\vw}{\sqrt{\vw^T\mS\vw}}
\end{equation}
By the definition of $E$ and its enclosure in the convex hull of the points we can write:
\begin{equation}
    \vy_w = \sum_i \lambda_i \vs^{[i]} \quad \lambda_i > 0, \sum_i \lambda_i  \leq 1
\end{equation}
Now:
\begin{equation}
    \vw^T\vy = \sqrt{\vw^T\mS\vw} = \sum_i \lambda_i \vw^T\vs^{[i]} \leq \max_i \vw^T\vs^{[i]} \sum_i \lambda_i = \max_i \vw^T\vs^{[i]}
\end{equation}
Therefore, we get our our main result:
\begin{equation}
    (\max_i\vw^T\vs^{[i]})^2 \geq \vw^T\mS\vw
\end{equation}

\subsubsection{Necessity of Condition}

Now we will show the necessity of this condition. We will do this by showing that if one of the points in $E$ is not within the convex hull of the datapoints then we can find one of the inequalities in \cref{eqn:max_inequality} that is broken.

First, get all the datapoints that for some unit vector $\vw$ maximise $\vw^T\vs^{[i]}$ over the dataset. Construct the convex hull of these points, the polyhedron $P$. You can equivalently characterise any polyhedra by a set of linear inequalities: $P = \{\vx\in\mathbb{R} :\mB\vx\leq \vb\}$. Denote with $\mB_j$ the jth row of $\mB$. We can always choose to write the inequalities in such a way that the rows of $\mB$ are unit length, by appropriately rescaling each $b_j$. Assume we have done this.

\begin{figure}
    \centering
    \includegraphics[width=0.5\linewidth]{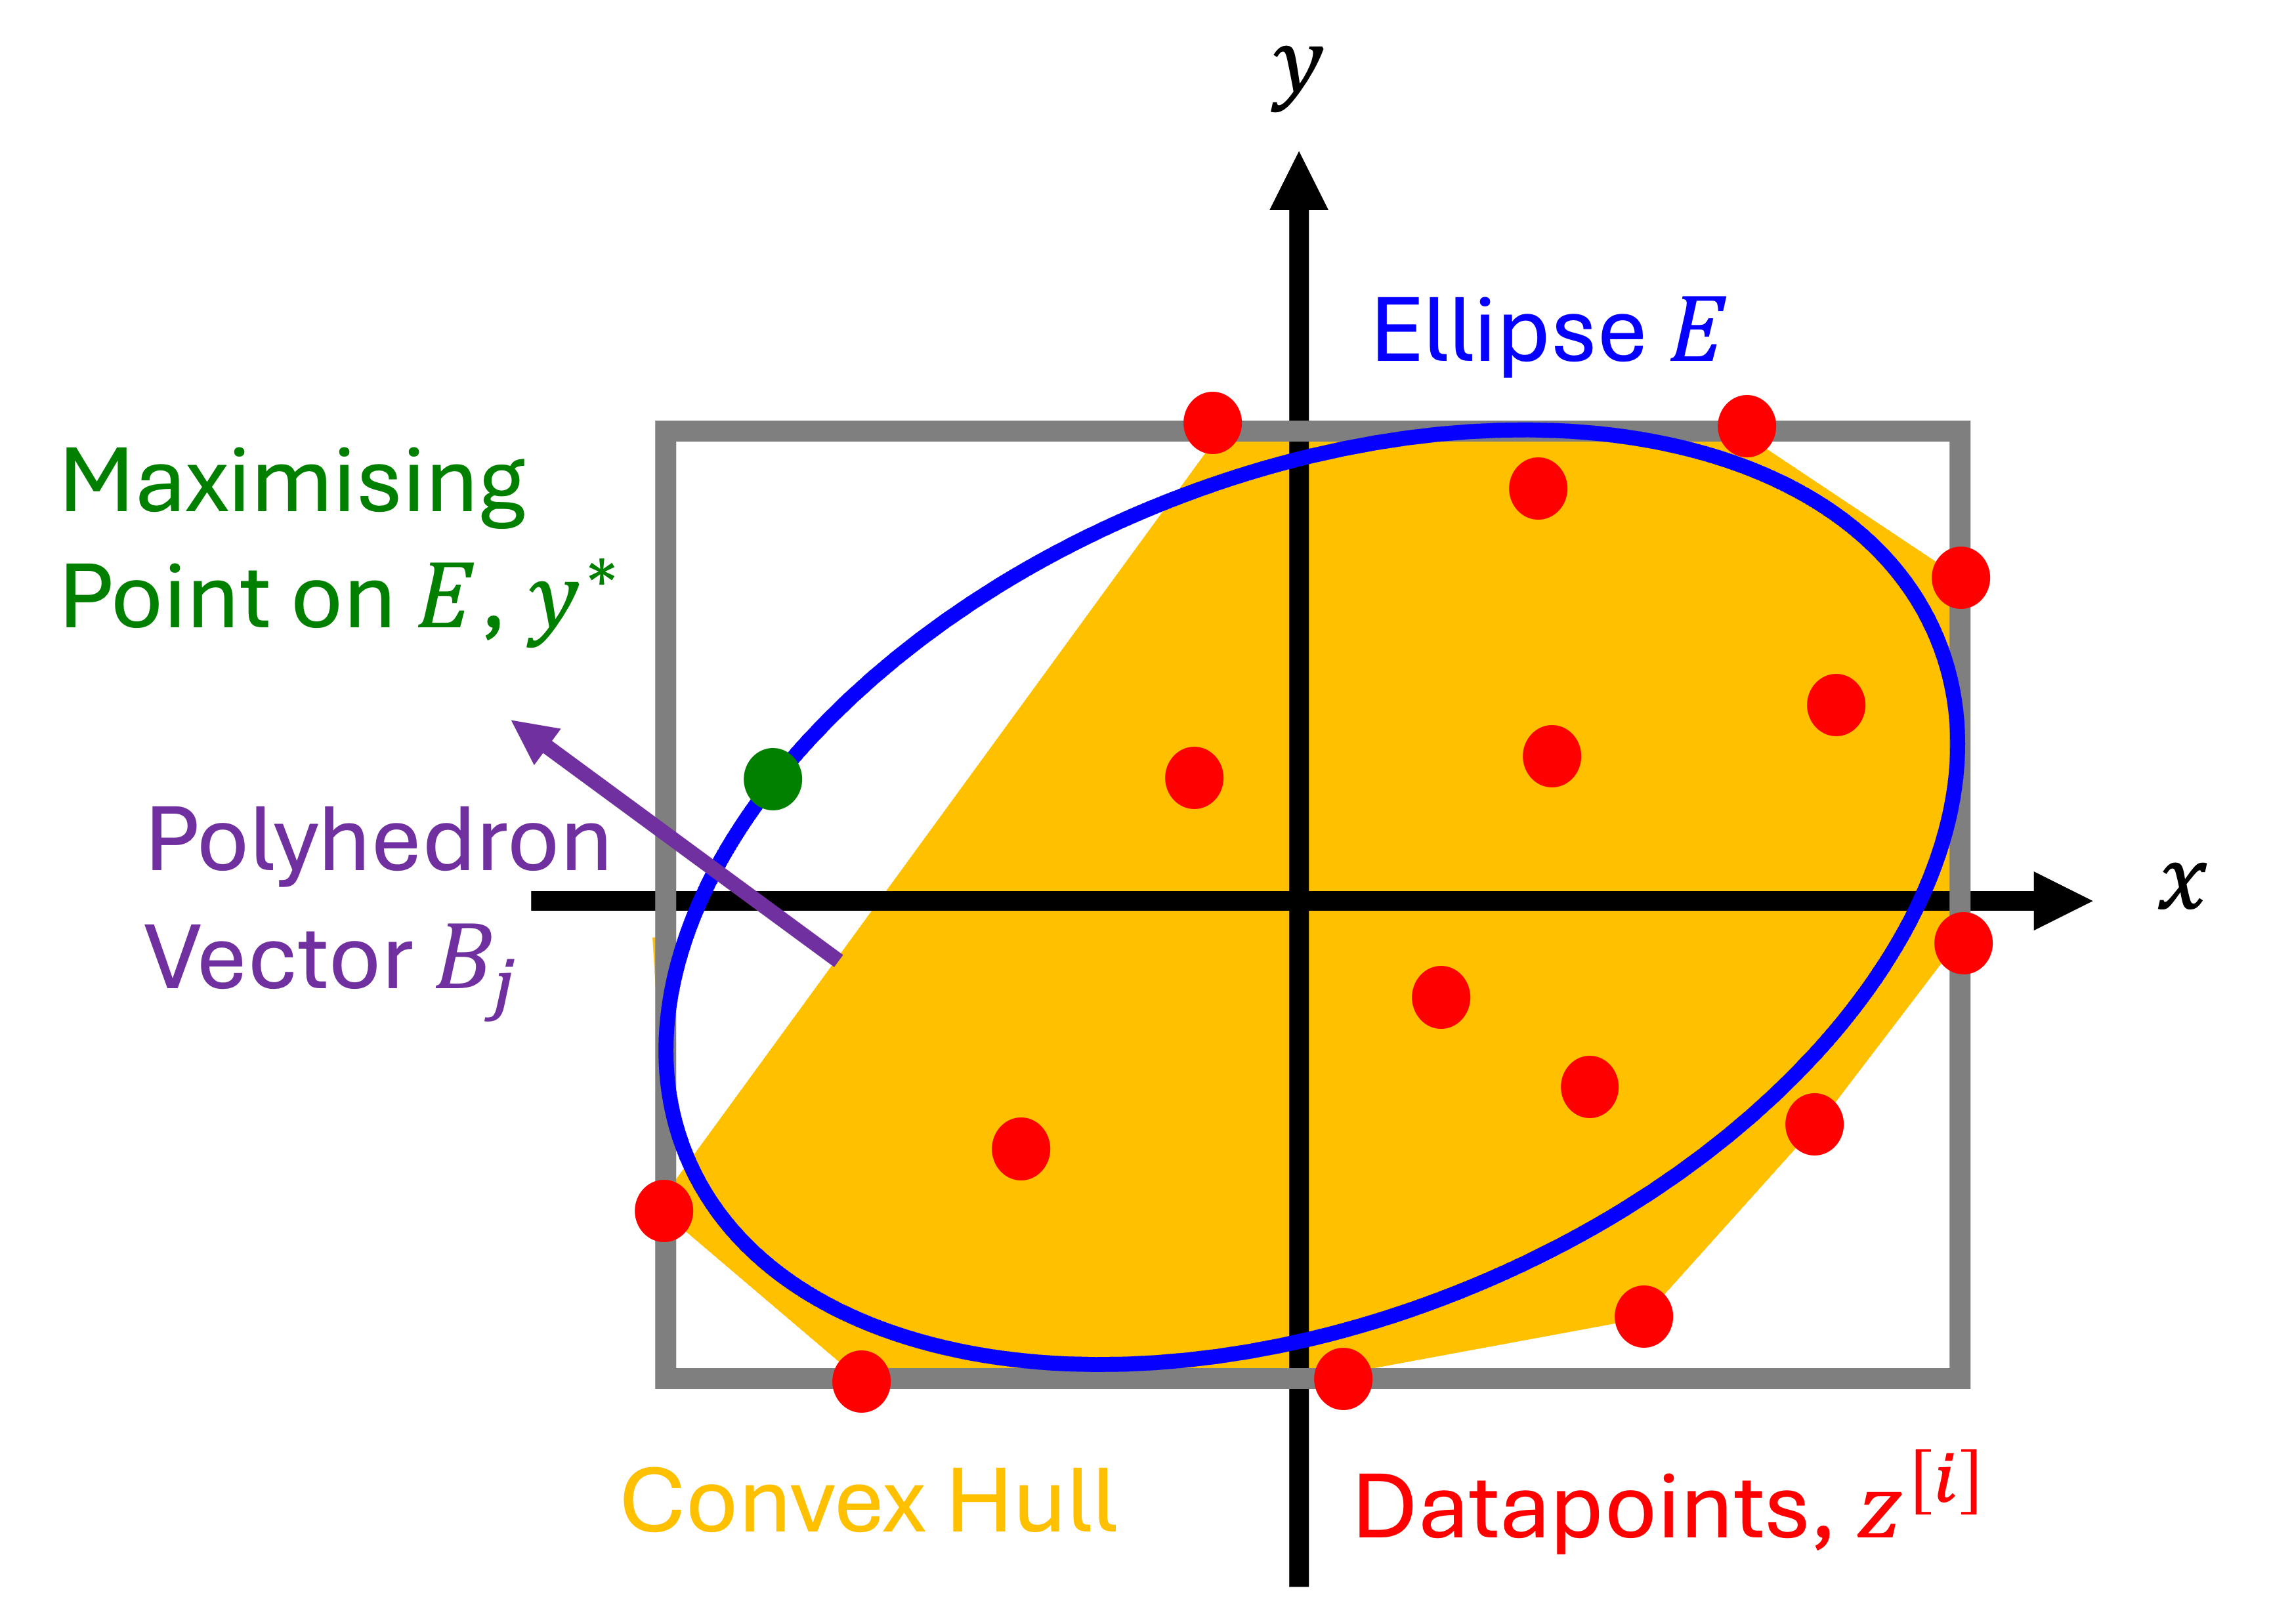}
    \caption{If the convex hull does not enclose the ellipse then you can always find a unit vector that breaks the inequality. In particular, this is true for the unit vector that defines the faces of the convex hull, $\mB_j$.}
    \label{fig:ellipse_proof_help}
\end{figure}

Assume the convex hull does not contain the entire ellipse. Therefore there is at least one point on the ellipse that breaks one of the inequalities defining the polyhedron. These points are charactersied by being both on the ellipse, $\vy^T\mS^{-1}\vy = 1$, but at least one of the inequalities defining the polyhedron is broken: $\mB_j^T\vy > b_j$. Let's call the set of points on the ellipse for which this inequality is broken $\mathcal{B}_j = \{\vy \in\mathbb{R}^n: \vy^T\mS^{-1}\vy = 1\quad \text{and} \quad \mB_j^T\vy > b_j\}$.

Now, choose the element of $\mathcal{B}_j$ that maximises $\mB_j^T\vy$, call it $\vy^*$. This will also be the element of $E$ that maximises $\mB_j^T\vy$, which by the previous lagrange optimisation, \cref{eq:lagrange_ellipse}, has the following dot product: $\mB_j^T\vy^* = \sqrt{\mB_j^T\mS\mB_j}$.

But now we derive a contradiction. This point is outside the polyhedron, $\mB_j^T\vy > b_j$, whereas all points inside the polyhedron, including all the datapoints, satisfy all inequalities, hence, $\mB_j^T\vs^{[i]} \leq b_j \forall \vs^{[i]}$. But, $\mB_j^T\vy^* = \sqrt{\mB_j^T\mS\mB_j} > b_j$, therefore:
\begin{equation}
    \mB_j^T\vs^{[i]} \leq b_j < \sqrt{\mB_j^T\mS\mB_j}\quad  \forall \vs^{[i]}
\end{equation}
And hence we've found a unit vector $\mB_i$ such that:
\begin{equation}
    \max_i \mB_j^T\vs^{[i]} < \sqrt{\mB_j^T\mS\mB_j} \quad \rightarrow \quad (\max_i \mB_j^T\vs^{[i]})^2 < \mB_j^T\mS\mB_j
\end{equation}
Hence one of the inequalities in $\cref{eqn:max_inequality}$ is broken, showing the necessity.

\subsubsection{Generalisation to Linearly Mixed Sources}

Using an exactly analogous strategy, one can show that, in the setting of \cref{thm:linearly_mixed_sources}, an equivalent condition for the set of inequalities to be satisfied, is for the convex hull of the datapoints to contain the ellipse $E = \{\vy: \vy^T\mS^{-1}\vy\}$, where:
\begin{equation}
    \mS = \lambda\mD^{-2}(\mA^T\mA)\mD^{-2} - \lambda(\mA^T\mA)^{-1} -\langle \vs^{[i]}(\vs^{[i]})^T\rangle_i
\end{equation}

\section{Extension to all Activity Norms}\label{app:other_activity_norms}

We now extend our theoretical results to the same setting as the main theorem, \cref{thm:linear_autoencoding_app}, but with other activity norms rather than L2. As shown in theorem~\cref{thm:weight_loss_minimised_by_modularising}, the weight loss is minimised by orthogonalising the coding of different variables, so we just focus on the activity loss and will recombine later. We will show that, for all norms, modular solutions are optimal if the variables are range independent. 

Consider a set of modular neurons:
\begin{equation}
    \vz_n^{[i]} = \begin{bmatrix}|u_{n1}|(\bar{s}_1^{[i]}- \min_j \bar{s}_{1}^{[j]})\\ \vdots \\ |u_{nd_{s}}|(\bar{s}_{d_s}^{[i]}-\min_j\bar{s}_{d_s}^{[i]}) \end{bmatrix}\geq {\bf 0}
\end{equation}
And let's see if we could usefully mix these encodings together for any set of mixing coefficients $\vu_n\in\mathbb{R}^{d_s}$:
\begin{equation}
    z_n^{[i]} = \sum_{j=1}^{d_s} u_{nj}\bar{s}_j^{[i]} + \Delta_n = \sum_{j=1}^{d_s} u_{nj}\bar{s}_j^{[i]} - \min_i[\sum_{j=1}^{d_s} u_{nj}\bar{s}_j^{[i]}] \geq 0
\end{equation}
If the variables are range-independent then we can move the min inside the sum:
\begin{equation}
    \Delta_n = - \min_i[\sum_{j=1}^{d_s} u_{nj}\bar{s}_j^{[i]}] = -\sum_{j=1}^{d_s} \min_iu_{nj}\bar{s}_j^{[i]}
\end{equation}
Then the Lp norm is:
\begin{equation}
    \langle |z_n^{[i]}|^p\rangle_i = \langle |\bigg(\sum_{j=1}^{d_s} u_{nj}\bar{s}_j^{[i]} + \Delta_n\bigg)|^p\rangle_i = \langle |\bigg(\sum_{j=1}^{d_s} u_{nj}\bar{s}_j^{[i]} -\min_iu_{nj}\bar{s}_j^{[i]}\bigg)|^p\rangle_i
\end{equation}
Now using the convexity of the Lp norm:
\begin{equation}
    \langle |\bigg(\sum_{j=1}^{d_s} u_{nj}\bar{s}_j^{[i]} -\min_iu_{nj}\bar{s}_j^{[i]}\bigg)|^p\rangle_i \geq \sum_{j=1}^{d_s} \langle |u_{nj}\bar{s}_j^{[i]} -\min_iu_{nj}\bar{s}_j^{[i]}|^p\rangle_i
\end{equation}
with equality only if p is equal to 1, or if at most one of the entries of $\vu$ are 0.

Finally, since we orient our variables such that $|\min_i \bar{s}^{[i]}_j| < \max_i \bar{s}^{[i]}$, without loss of generality,:
\begin{equation}
    \langle |u_{nj}\bar{s}_j^{[i]} -\min_iu_{nj}\bar{s}_j^{[i]}|^p\rangle_i \geq \langle |u_{nj}|^p\langle|\bar{s}_j^{[i]} -\min_i\bar{s}_j^{[i]}|^p\rangle_i
\end{equation}
So we get our final result that the mixed activity loss is greater than or equal to the modular activity loss if the variables are range independent:
\begin{equation}
    \langle |z_n^{[i]}|^p\rangle_i \geq \sum_{j=1}^{d_s}|u_{nj}|^p\langle|\bar{s}_j^{[i]} -\min_i\bar{s}_j^{[i]}|^p\rangle_i = \langle |\vz_n^{[i]}|^p\rangle_i
\end{equation}
So, as long as $p>1$, the activity loss is lowered by modularising the representation of range-independent variables. Further, since the weight loss is also minimised, the optimal solution will be modular.

Two caveats: first, in the particular case of the L1 norm all that we can guarantee is that the activity loss of a modular solution is equal to that of a mixed solution. This means that, even in the case of range-independent variables, there might be orthogonal but mixed solutions that are equally good as the modular solution. For $p>1$ this caveat is not needed.

Second, this is a set of sufficient conditions, range-independent variables are optimally encoded modularly. There will be other nearly range-independent variables that are also optimally encoded modularly, just as we found for the L2 case.

\section{Extension to Multidimensional Variables}\label{app:multi_dimensional_vars}

Many variables in the real world, such as angles on a circle, are not 1-dimensional. Ideally our theory would tell us when such multi-dimensional sources were modularised. Unfortunately, precise necessary and sufficient conditions are not an easy step from our current theory because our proof strategies make extensive use of the optimal modular encoding. For one-dimensional sources this is very easy to find, simply align each source correctly in a neuron, and make the representation positive. Finding similar optimal modular solutions for multidimensional sources is much harder, potentially as hard as simply solving the optimisation problem. 

However, we can make progress on a simpler problem: showing that range-independence is a sufficient condition for a set of multi-dimensional sources to modularise. Consider two multidimensional sources $\vx^{[i]}\in\mathbb{R}^{d_x}$ and $\vy^{[i]}\in\mathbb{R}^{d_y}$, and an encoding in which they are mixed in single neurons:
\begin{equation}
    z_n^{[i]} = \sum_{j=1}^{d_x}u_{nj}x_j^{[i]} + \sum_{j=1}^{d_y}v_{nj}y_j^{[i]} + \Delta_n
\end{equation}
Whatever choice of coefficient vectors, $\vu$ and $\vv$, or activity norm (as long as $p>1$), we can consider breaking this mixed coding into two modular neurons. Define new variables $a^{[i]} = \sum_{j=1}^{d_x}u_{nj}x_j^{[i]}$ and $b^{[i]} = \sum_{j=1}^{d_y}v_{nj}y_j^{[i]}$. If the two multidimensional sources are range-independent, then so too are $a$ and $b$. Define the modular representation:
\begin{equation}
    \vz_n^{[i]} = \begin{bmatrix}
        a^{[i]} - \min_j a^{[j]}\\        b^{[i]} - \min_j b^{[j]}
    \end{bmatrix}
\end{equation}
All of our previous arguments apply to argue that this modular encoding will be preferred if the multidimensional variables are range-independent.

We just have to show that the weight loss is also reduced by modularising multidimensional sources, a small extension of \cref{thm:weight_loss_minimised_by_modularising}, which we shall now show. Write a modular code as:
\begin{equation}
    \vz^{[i]} =
    \mU \vx^{[i]} - \min_j [\mU \vx^{[j]}] +   \mV \vy^{[i]} - \min_j [\mV \vy^{[j]}]
\end{equation}
With the encoding of $\vx$ and $\vy$ spanning two different spaces: $\mU^T\mV = {\bf 0}$.

Then define the minimal L2 norm readout weight matrix using the pseudoinverse:
\begin{equation}
    \mW_{\text{out}} = \begin{bmatrix}
        \mU^{\dagger}\\\mV^{\dagger}
    \end{bmatrix}
\end{equation}
Such that $\mW_{\text{out}}\vz^{[i]} = \begin{bmatrix}
    \vx^{[i]} \\ \vy^{[i]} 
\end{bmatrix}$ up to some constant offset that can be removed by the bias term in the readout. Now consider mixing the representation of the two multidimensional sources using an orthogonal matrix that preserves the encoding size of each variable, $\mO$:
\begin{equation}
    \vz^{[i]} = \mU\vx^{[i]} + \mO\mV\vy^{[i]} \qquad \mW_{\text{out}} =     \mW_{\text{out}} = \begin{bmatrix}
        \mU^\dagger + \mA\\ \mV^\dagger\mO^T+ \mB
    \end{bmatrix}
\end{equation}
Then in the subspace spanned by the columns of $\mU$ $\mW_{\text{out}}$ must be the same as $\mU^{\dagger}$. However, in order to offset the newly aligned matrix $\mO\tilde{\mV}$ there must be an additional component orthogonal, $\mA$:
\begin{equation}
\begin{aligned}
    \mW_{out}\mU = \mU^{\dagger}\mU + \mA\mU = \mathbb{I} \qquad \mA\mU = {\bf 0} \\
    \mW_{out}\mO\mV = \mU^{\dagger}\mO\mV + \mA\mO\mV = {\bf 0} \qquad \mA\mO\mV = -\mU^{\dagger}\mO\mV
\end{aligned}
\end{equation}
So $\mA$ and $\mU^\dagger$ live in orthogonal subspaces, and $\mA \neq 0$. The same applies to $\mV$ and $\mB$, therefore:
\begin{equation}
    ||\mW_{out}||_F^2 = ||\mU^{\dagger}||_F^2 + ||\mV^{\dagger}||_F^2  + ||\mA||_F^2 + ||\mB||_F^2 \geq ||\mU^{\dagger}||_F^2 + ||\mV^{\dagger}||_F^2
\end{equation}
And hence orthogonalising the subspaces reduces the loss in this case as well.

Combining these two, the optimal representation of range-independent multi-dimensional variables for activity losses using an Lp norm for $p>1$ is modular.
